# Supplementary material for: GCformer: An Efficient Framework for Accurate and Scalable Long-Term Multivariate Time Series Forecasting
Source: arXiv:2306.08325 source file (2023-08-15)
Supplement: Supplementary file 1 [file 6_Appendix.tex]

\section{Related Work}
\label{App:related_works}
In this section, we will give an overview of the related literature in time series forecasting. %The relevant work includes traditional times series models (\ref{App:related_work_tradi_time}), deep learning models (\ref{App:related_work_tradi_time}), Transformer-based models (\ref{App:related_work_transformers}), and the Fourier Transform in neural networks (\ref{App:related_work_fft}).

% \subsection{General Time-line of Time Series Models}
% \label{App:related_work_tradi_time}

%Data-driven time series forecasting helps researchers understand the evolution of the systems without architecting the exact physics law behind them. After decades of renovation, time series models have been well developed and served as the backbone of various projects in numerous application fields. 

\paragraph{Traditional Time Series Models} The first generation of well-discussed time series model is the autoregressive family. ARIMA~\cite{box_arima2,box_distribution_1970} follows the Markov process and build recursive sequential forecasting. However, a plain autoregressive process has difficulty in dealing non-stationary sequences. Thus, ARIMA employed a pre-process iteration by differencing, which transforms the series to stationary. Still, ARIMA and related models have the linear assumption in the autoregressive process, which limits their usage in complex forecasting tasks. 

\paragraph{Deep Neural Network in Forecasting}
With the bloom of deep neural networks, recurrent neural networks (RNNs) were designed for tasks involving sequential data. However, canonical RNN tends to suffer from gradient vanishing/exploding problems with long input because of its recurrent structure. Among the family of RNNs, LSTM~\cite{hochreiter_long_1997_lstm} and GRU~\cite{GRU_cho_et_al_2014} proposed gated structure to control the information flow to deal with the gradient vanishing/exploration problem. Although recurrent networks enjoy fast inference, they are slow to train and not parallelizable. Temporal convolutional network (TCN)~\cite{Think_globally_act_locally_tcn_time_series_2019} is another family for sequential tasks. However, limited to the reception field of the kernel, the long-term dependencies are hard to capture. Convolution is a parallelizable operation but expensive in inference.

\paragraph{Transformers}
With the innovation of Transformers in natural language processing~\cite{attention_is_all_you_need,Bert/NAACL/Jacob} and in computer vision tasks~\cite{Transformers-for-image-at-scale/iclr/DosovitskiyB0WZ21,DBLP:Global-filter-FNO-in-cv}, they are also discussed, renovated, and applied in time series forecasting~\cite{wen2022transformers}, especially the main attention module. Some works use temporal attention~\cite{dual-state-attention-rnn-qin} to capture long-range dependencies for time series. Others use the backbone of Transformer. Transformers usually employ an encoder-decoder architecture, with the self-attention and cross-attention mechanisms serving as the core layers. \cite{Log-transformer-shiyang-2019} invents a logsparse attention module to deal with the memory bottleneck for Transformer model. \cite{DBLP:conf/iclr/KitaevKL20-reformer} uses locality-sensitive
hashing to replace the attention module for less time complexity. \cite{haoyietal-informer-2021} proposes a probability sparse attention mechanism to deal with long-term forecasting. \cite{Autoformer} designs a decomposition Transformer architecture with an Auto-Correlation mechanism as an alternative for the attention module. \cite{liu2022pyraformer} designs a low-complexity Pyramidal Attention for the long-term time forecasting tasks. \cite{FedFormer} proposes two attention modules that operate in the frequency domain using Fourier or wavelet transformation.

\paragraph{Orthogonal Basis and Neural Network}
Orthogonal basis project arbitrary functions onto a certain space and thus enable the representation learning in another view. Orthogonal basis family is easy to be discretized and serves as a plug-in operation in neural networks. Recent studies began to realize the efficiency and effectiveness of the Orthogonal basis, including the polynomial family and others (Fourier basis \& Multiwavelet basis). Fourier basis is first introduced for acceleration due to the Fast Fourier algorithm, for example, acceleration of computing convolution~\cite{Hippo} or Auto-correlation function~\cite{wen2021robustperiod,Autoformer}. Fourier basis also serves as a performance boosting block: Fourier with Recurrent structure~\cite{FourierRecurrentUnits}, Fourier with MLP~\cite{Fourier-Neural-Operator,FNet} and Fourier in Transformer~\cite{FedFormer}. Multiwavelet transform is a more local filter (compared with 
Fourier) and a frequency decomposer. Thus, neural networks which employ multiwavelet filter usually exhibit a hierarchical structure and treat different frequency in different tunnels, e.g., \cite{wang2018multilevel,Multiwavelet-based-Operator-Learning,FedFormer}. Orthogonal Polynomials are naturally good selections of orthogonal basis. Legendre Memory Unit (LMU)~\cite{LMU} uses Legendre Polynomials for an orthogonal projection of input signals for memory strengthening with the backbone of LSTM. The projection process is mathematically derived from delayed linear transfer function. HiPPO~\cite{Hippo}, based on LMU, proposes a novel mechanism (Scaled Legendre), which involves the function's full history (LMU uses rolling windowed history). In the subsequent work of HiPPO, the authors propose S4 model~\cite{S4} and give the first practice on time series forecasting tasks. However, LMU and HiPPO share the same backbone (LSTM), which may limit their performance. %Furthermore, the setting of Scale Legendre in HiPPO (history without decay) may not stand in time series forecasting.

% Legendre

% Laguerre

% ~\cite{FNet}

% \subsection{State Space Model}
% RFF is compact in \cite{Sampled-softmax-with-random-Fourier-Features/nips/RawatCYSK19}

% Optimal Rates for Random Fourier Features

\section{Algorithm Implementation}
\label{app:Alg}
\input{figures/algorithm_0}
%\paragraph{Implementation for Frequency Enhanced Layer}
\input{figures/algorithm_1}
\section{Dataset and Implementation Details}
\label{app:section_dataset_implem}
\subsection{Dataset Details}
\label{app:dataset}
In this subsection, we summarize the details of the datasets used in this paper as follows: 1) ETT~\cite{haoyietal-informer-2021} dataset contains two sub-dataset: ETT1 and ETT2, collected from two separated counties. Each of them has two versions of sampling resolutions (15min \& 1h). ETT dataset contains multiple time series of electrical loads and one time sequence of oil temperature. 2) Electricity\footnote{https://archive.ics.uci.edu/ml/datasets/ElectricityLoadDiagrams 20112014} dataset contains the electricity consumption for more than three hundred clients with each column corresponding to one client. 3) Exchange~\cite{lai2018modeling-exchange-dataset} dataset contains the current exchange of eight countries. 4) Traffic\footnote{http://pems.dot.ca.gov} dataset contains the occupation rate of freeway systems in California, USA. 5) Weather\footnote{https://www.bgc-jena.mpg.de/wetter/} dataset contains 21 meteorological indicators for a range of one year in Germany. 6) Illness\footnote{https://gis.cdc.gov/grasp/fluview/fluportaldashboard.html} dataset contains the influenza-like illness patients in the United States. Table \ref{tab:dataset} 
\input{tables/tab_dataset}
summarizes all the features of the six benchmark datasets. They are all split into the training set, validation set, and test set by the ratio of 7:1:2 during modeling.

\subsection{Implementation Details}
\label{app:exp:implement}
Our model is trained using ADAM \cite{kingma_adam:_2017} optimizer with a learning rate of $1e^{-4}$ to  $1e^{-3}$. The batch size is set to 32 (It depends on the GPU memory used in the experiment. In fact, a batch size up to 256 does not deteriorate the performance but with faster training speed if larger memory GPU or multiple GPUs is used). The default training process is 15 epochs without any early stopping. We save the model with the lowest loss on the validation set for the final testing. The mean square error (MSE) and mean absolute error (MAE) are used as metrics. All experiments are repeated 5 times and the mean of the metrics is reported as the final results. All the deep learning networks are implemented using PyTorch \cite{NEURIPS2019_9015_pytorch} and trained on NVIDIA V100 32GB GPUs/NVIDIA V100 16GB GPUs.

\subsection{Experiment Error Bars}
We train our model 5 times and calculate the error bars for FiLM and SOTA model FEDformer to compare the robustness, which is summarized in Table~\ref{tab:std}. It can be seen that the overall performance of the proposed FiLM is better than that of the SOTA FEDformer model.

\label{app:error_bars}
\vspace{-.2cm}
\begin{table}[ht]
%\setlength{\uppercaptionskip}{0.pt}
%\setlength{\belowcaptionskip}{-0.pt}
% \label{sample-table-kstest}
%\vskip 0.15in
\centering
\caption{MSE with error bars (Mean and STD) for FiLM and FEDformer baseline for multivariate long-term forecasting. All experiments are repeated 5 times.}
\begin{small}
% \begin{sc}
\scalebox{0.75}{
\begin{tabular}{c|c|ccccc}
\toprule
\multicolumn{2}{c|}{MSE}& ETTm2 & Electricity & Exchange & Traffic\\ %&\multicolumn{2}{c|}{Fedformer-f }\\%&\multicolumn{2}{c|}{}&\\
\midrule
\multirow{4}{*}{\rotatebox{90}{FiLM}} 
& 96 & 0.165 $\pm$ 0.0051 & 0.153$\pm$ 0.0014 & 0.079$\pm$ 0.002 & 0.416$\pm$ 0.010 \\
& 192 & 0.222 $\pm$ 0.0038 & 0.165$\pm$ 0.0023 & 0.159$\pm$ 0.011 & 0.408$\pm$ 0.007 \\
& 336 & 0.277 $\pm$ 0.0021 & 0.186$\pm$ 0.0018 & 0.270$\pm$ 0.018 & 0.425$\pm$ 0.007 \\
& 720 & 0.371 $\pm$ 0.0066 & 0.236$\pm$ 0.0022 & 0.536$\pm$ 0.026 & 0.520$\pm$ 0.003 \\
\midrule
\multirow{4}{*}{\rotatebox{90}{FED-f}} 
& 96 & 0.203 $\pm$ 0.0042 & 0.194 $\pm$ 0.0008 & 0.148 $\pm$ 0.002 & 0.217 $\pm$ 0.008 \\
& 192 & 0.269 $\pm$ 0.0023 & 0.201$\pm$ 0.0015 & 0.270$\pm$ 0.008 & 0.604 $\pm$ 0.004 \\
& 336 & 0.325 $\pm$ 0.0015 & 0.215$\pm$ 0.0018 & 0.460$\pm$ 0.016 & 0.621 $\pm$ 0.006 \\
& 720 & 0.421 $\pm$ 0.0038 & 0.246$\pm$ 0.0020 & 1.195$\pm$ 0.026 & 0.626 $\pm$ 0.003 \\
\bottomrule
\end{tabular}
}
\label{tab:std}
% \end{sc}
\end{small}
%\end{center}
\vskip -0.1in
\end{table}

\subsection{Univariate Forecasting Results}
\label{app:exp:uni_bench}
The univariate benchmark results are summarized in Table~\ref{tab:uni-benchmarks-large}.
\begin{table*}[h]
% \begin{adjustwidth}{-1.5in}{-1in}
\centering
%\begin{small}
\caption{Univariate long-term forecasting results on six datasets with various input length and prediction horizon $O \in \{96,192,336,720\}$. A lower MSE indicates better performance. All experiments are repeated 5 times.}
\vskip 0.05in
\scalebox{0.60}{
\begin{tabular}{c|c|cccccccccccccc}
\toprule
\multicolumn{2}{c|}{Methods}&\multicolumn{2}{c|}{FiLM}&\multicolumn{2}{c|}{FEDformer}&\multicolumn{2}{c|}{Autoformer}&\multicolumn{2}{c|}{S4}&\multicolumn{2}{c|}{Informer}&\multicolumn{2}{c|}{LogTrans}&\multicolumn{2}{c}{Reformer}\\
\midrule
\multicolumn{2}{c|}{Metric} & MSE  & MAE & MSE & MAE& MSE  & MAE& MSE  & MAE& MSE  & MAE& MSE  & MAE& MSE  & MAE\\
\midrule
\multirow{4}{*}{\rotatebox{90}{$ETTm2$}} 
& 96 & 0.065 &\textbf{0.189}  &\textbf{0.063} &0.189 & 0.065 & 0.189 &0.153 &0.318 & 0.088 & 0.225 & 0.075 & 0.208 & 0.076  &0.214   \\
& 192 & \textbf{0.094} & \textbf{0.233} &0.102 &0.245 & 0.118 & 0.256 &0.183 &0.350 & 0.132 &0.283 & 0.129 &0.275  & 0.132  & 0.290   \\
& 336 & \textbf{0.124} & \textbf{0.274} &0.130 &0.279 & 0.154 & 0.305 &0.204 & 0.367 &0.180 &0.336 & 0.154 &0.302  & 0.160  & 0.312    \\
& 720 & \textbf{0.173} & \textbf{0.323} &0.178 &0.325 & 0.182 &0.335 &0.482 &0.567  &0.300  &0.435 & 0.160 &0.321  & 0.168  &0.335     \\
\midrule
\multirow{4}{*}{\rotatebox{90}{$Electricity$}} 
& 96  & \textbf{0.154} & \textbf{0.247} &0.253 &0.370  &0.341 &0.438 &0.351 &0.452 & 0.484& 0.538 &0.288& 0.393& 0.274 & 0.379   \\
& 192 & \textbf{0.166} & \textbf{0.258} &0.282 &0.386 &0.345 &0.428 &0.373 &0.455 & 0.557& 0.558 &0.432 & 0.483 & 0.304 &0.402   \\
& 336 & \textbf{0.188} & \textbf{0.283} &0.346 &0.431 &0.406 &0.470 &0.408 &0.477 & 0.636& 0.613 &0.430 &0.483 & 0.370 &0.448  \\
& 720 & \textbf{0.249} & \textbf{0.341} &0.422 &0.484 &0.565 &0.581 &0.472 &0.517 & 0.819& 0.682 &0.491 &0.531 & 0.460 &0.511   \\
\midrule

\multirow{4}{*}{\rotatebox{90}{$Exchange$}} 
&96  & \textbf{0.110} & \textbf{0.259} &0.131 &0.284 & 0.241 & 0.387 &0.344 &0.482  & 0.591  &0.615  &0.237 &0.377  &0.298  &0.444    \\
& 192 & \textbf{0.207} & \textbf{0.352} &0.277 &0.420 &0.300  &0.369 &0.362 &0.494  &1.183   &0.912 &0.738  &0.619  &0.777  & 0.719   \\
& 336 & \textbf{0.327} & \textbf{0.461} &0.426 &0.511 &0.509  &0.524 &0.499 &0.594  &1.367  &0.984  &2.018  &1.070  &1.832  &1.128     \\
& 720 & \textbf{0.811} & \textbf{0.708} &1.162 &0.832 &1.260  &0.867 &0.552 & 0.614 &1.872  &1.072  &2.405  &1.175  &1.203  &0.956     \\
\midrule
\multirow{4}{*}{\rotatebox{90}{$Traffic$}} 
&96  & \textbf{0.144} & \textbf{0.215} &0.170 &0.263  &0.246 &0.346 &0.194 &0.290 & 0.257 & 0.353 &0.226 &0.317 &  0.313 & 0.383\\
& 192 & \textbf{0.120} & \textbf{0.199} &0.173 &0.265 &0.266 &0.370 &0.172 &0.272 & 0.299 & 0.376 &0.314 &0.408 & 0.386 & 0.453\\
& 336 & \textbf{0.128} & \textbf{0.212} &0.178 &0.266 &0.263 &0.371 &0.178 &0.278 & 0.312 & 0.387 &0.387 &0.453 & 0.423 & 0.468\\
& 720 & \textbf{0.153} & \textbf{0.252} &0.187 &0.286 &0.269 &0.372 &0.263 &0.386 & 0.366 & 0.436 &0.491 &0.437 & 0.378 & 0.433\\
\midrule
\multirow{4}{*}{\rotatebox{90}{$Weather$}}
& 96  & \textbf{0.0012} & \textbf{0.026} & 0.0035 & 0.046 & 0.011 &0.081 &0.0061 &0.065 & 0.0038 & 0.044 & 0.0046 &0.052 & 0.012 & 0.087 \\
& 192 & \textbf{0.0014}& \textbf{0.029}&0.0054 &0.059 &0.0075 &0.067 &0.0067 &0.067 & 0.0023 & 0.040 &0.0056 & 0.060 & 0.0098 & 0.079  \\
& 336 & \textbf{0.0015} & \textbf{0.030} &0.0041 &0.050 &0.0063 &0.062 &0.0025 &0.0381 & 0.0041 & 0.049 &0.0060 &0.054& 0.0050 & 0.059 \\
& 720 & \textbf{0.0022} & \textbf{0.037} &0.015 &0.091 &0.0085 &0.070 &0.0074 &0.0736 & 0.0031 & 0.042 &0.0071 &0.063& 0.0041 & 0.049 \\
\midrule
\multirow{4}{*}{\rotatebox{90}{$ILI$}} 
& 24 & \textbf{0.629} & \textbf{0.538} &0.693 &0.629 &0.948 &0.732 &0.866 &0.584 & 5.282 &2.050 &3.607 & 1.662 & 3.838 & 1.720  \\
& 36 & \textbf{0.444} & \textbf{0.481} &0.554 &0.604 &0.634 &0.650 &0.622 &0.532 & 4.554 &1.916 &2.407 & 1.363 & 2.934 & 1.520 \\
& 48 & \textbf{0.557} & \textbf{0.584} &0.699 &0.696 &0.791 &0.752 &0.813 &0.679 & 4.273 &1.846 &3.106 & 1.575 & 3.754 & 1.749\\
& 60 & \textbf{0.641} & \textbf{0.644} &0.828 &0.770 &0.874 &0.797 &0.931 &0.747 & 5.214 &2.057 &3.698 & 1.733 & 4.162 & 1.847\\
\bottomrule
\end{tabular}
}
\label{tab:uni-benchmarks-large}
\vskip -0.10in
% \end{adjustwidth}
%\end{small}tab:multi-benchmarks
\end{table*}

\subsection{ETT Full Benchmark}
\label{app:exp:ett_benchmark}
We present the full-benchmark on four ETT datasets \cite{haoyietal-informer-2021} in Table \ref{tab:multi-benchmarks-ett} (multivariate forecasting) and Table \ref{tab:uni-benchmarks-ett} (univariate forecasting). The ETTh1 and ETTh2 are recorded hourly while ETTm1 and ETTm2 are recorded every 15 minutes. The time series in ETTh1 and ETTm1 follow the same pattern, and the only difference is the sampling rate, similarly for ETTh2 and ETTm2. On average, our 
FiLM yields a \textbf{14.0\%} relative MSE reduction for multivariate forecasting, and a \textbf{16.8\%} reduction for univariate forecasting over the SOTA results from FEDformer.
\label{app:ETT}

\begin{table*}[h]
\centering
% \begin{small}
% \begin{adjustwidth}{-1.5in}{-1in}
\caption{Multivariate long-term forecasting results on ETT full benchmark. The best results are highlighted in bold. A lower MSE indicates better performance. All experiments are repeated 5 times.}
\vskip 0.05in
\scalebox{0.75}{
\begin{tabular}{c|c|cccccccccccccccccc}
\toprule
\multicolumn{2}{c|}{Methods}&\multicolumn{2}{c|}{FiLM}&\multicolumn{2}{c|}{FEDformer}&\multicolumn{2}{c|}{Autoformer}&\multicolumn{2}{c|}{S4}&\multicolumn{2}{c|}{Informer}&\multicolumn{2}{c|}{LogTrans}&\multicolumn{2}{c}{Reformer}\\
\midrule
\multicolumn{2}{c|}{Metric} & MSE  & MAE & MSE & MAE& MSE  & MAE& MSE  & MAE& MSE  & MAE& MSE  & MAE& MSE  & MAE\\
\midrule
\multirow{4}{*}{\rotatebox{90}{$ETTh1$}}
& 96 &\textbf{0.371} &\textbf{0.394} &0.376 &0.419  & 0.449& 0.459 &0.949 &0.777 & 0.865 & 0.713& 0.878& 0.740& 0.837& 0.728\\
& 192 &\textbf{0.414} &\textbf{0.423} &0.420 &0.448  & 0.500& 0.482 &0.882 &0.745 & 1.008 & 0.792& 1.037& 0.824& 0.923& 0.766\\
& 336 &\textbf{0.442} &\textbf{0.445} &0.459 &0.465  & 0.521& 0.496 &0.965 &0.75 & 1.107 & 0.809& 1.238& 0.932& 1.097& 0.835\\
& 720 &\textbf{0.465} &\textbf{0.472} &0.506 &0.507  & 0.514& 0.512 &1.074&0.814 & 1.181 &0.865&  1.135& 0.852& 1.257& 0.889\\
\midrule
\multirow{4}{*}{\rotatebox{90}{$ETTh2$}}
& 96  &\textbf{0.284} &\textbf{0.348} &0.346 &0.388 & 0.358& 0.397 &1.551&	0.968 & 3.755& 1.525& 2.116& 1.197 &2.626 &1.317\\
& 192 &\textbf{0.357} &\textbf{0.400} &0.429 &0.439 & 0.456& 0.452 &2.336	 &1.229 & 5.602& 1.931& 4.315& 1.635 &11.12 &2.979\\
& 336 &\textbf{0.377} &\textbf{0.417} &0.482 &0.480 & 0.482& 0.486 &2.801	 &1.259 & 4.721& 1.835& 1.124& 1.604 &9.323 &2.769\\
& 720 &\textbf{0.439} &\textbf{0.456} & 0.463 & 0.474 & 0.515& 0.511 &2.973	 &1.333 & 3.647& 1.625& 3.188& 1.540 &3.874 &1.697\\
\midrule
\multirow{4}{*}{\rotatebox{90}{$ETTm1$}}
& 96  &\textbf{0.302} &\textbf{0.345} &0.378 &0.418 & 0.505& 0.475 &0.640	 &0.584 & 0.672& 0.571& 0.600& 0.546 &0.538 &0.528\\
& 192 &\textbf{0.338} &\textbf{0.368} & 0.426 & 0.441 & 0.553& 0.496 &0.570	 &0.555 & 0.795& 0.669& 0.837& 0.700 &0.658 &0.592\\
& 336 &\textbf{0.373} &\textbf{0.388} & 0.445 & 0.459 & 0.621& 0.537 &0.795& 0.691& 1.212& 0.871& 1.124& 0.832 &0.898 &0.721\\
& 720 &\textbf{0.420} &\textbf{0.420} & 0.543 & 0.490 & 0.671& 0.561 &0.738 &0.655 & 1.166& 0.823& 1.153& 0.820 &1.102 &0.841\\
\midrule
\multirow{4}{*}{\rotatebox{90}{$ETTm2$}} &96 &\textbf{0.165} &\textbf{0.256} & 0.203 & 0.287 &0.255  &0.339  &0.705	 &0.690  &0.365  &0.453  &0.768  &0.642  &0.658  &0.619 \\
                        & 192 &\textbf{0.222} &\textbf{0.296} & 0.269 & 0.328 &0.281 &0.340  &0.924	 &0.692 &0.533  &0.563  &0.989  &0.757  &1.078  &0.827 \\
                        & 336 &\textbf{0.277} &\textbf{0.333} & 0.325 & 0.366  &0.339  &0.372  &1.364	 & 0.877 &1.363&0.887  &1.334  &0.872  &1.549  &0.972 \\
                        & 720 &\textbf{0.371} &\textbf{0.389} & 0.421 & 0.415  &0.422  &0.419  &2.074 &1.074  &3.379  &1.338 & 3.048 &1.328  &2.631  &1.242 \\
\bottomrule
\end{tabular}
}
\label{tab:multi-benchmarks-ett}
% \end{adjustwidth}
% \end{small}
% \vskip -0.1in
\end{table*}

\begin{table*}[h]
\centering
% \begin{small}
% \begin{adjustwidth}{-1.5in}{-1in}
\caption{Univariate long-term forecasting results on ETT full benchmark. The best results are highlighted in bold. A lower MSE indicates better performance. All experiments are repeated 5 times.}
\vskip 0.05in
\scalebox{0.75}{
\begin{tabular}{c|c|cccccccccccccccccc}
\toprule
\multicolumn{2}{c|}{Methods}&\multicolumn{2}{c|}{FiLM}&\multicolumn{2}{c|}{FEDformer}&\multicolumn{2}{c|}{Autoformer}&\multicolumn{2}{c|}{S4}&\multicolumn{2}{c|}{Informer}&\multicolumn{2}{c|}{LogTrans}&\multicolumn{2}{c}{Reformer}\\
\midrule
\multicolumn{2}{c|}{Metric} & MSE  & MAE & MSE & MAE& MSE  & MAE& MSE  & MAE& MSE  & MAE& MSE  & MAE& MSE  & MAE\\
\midrule

\multirow{4}{*}{\rotatebox{90}{$ETTh1$}}
&96 &\textbf{0.055}&\textbf{0.178}&0.079 &0.215 &0.071 &0.206 &0.316 &0.490 &	0.193&	0.377&	0.283&	0.468&	0.532&	0.569\\
&192 &\textbf{0.072}&\textbf{0.207}&0.104 &0.245 & 0.114&	0.262 & 0.345&0.516 &	0.217&	0.395&	0.234&	0.409&	0.568&	0.575\\
&336 &\textbf{0.083}&\textbf{0.229}&0.119 &0.270 &0.107&0.258 &0.825 &0.846 &	0.202&	0.381&	0.386&	0.546&	0.635&	0.589\\
&720 &\textbf{0.090}&\textbf{0.240}&0.127 &0.280 &0.126&0.283 &0.190 &0.355 &	0.183&	0.355&	0.475&	0.628&	0.762&	0.666\\
\midrule
\multirow{4}{*}{\rotatebox{90}{$ETTh2$}}
&96 &\textbf{0.127}&0.272&0.128 &\textbf{0.271} & 0.153&	0.306 & 0.381&0.501 &	0.213&	0.373&	0.217&	0.379&	1.411&	0.838\\
&192 &\textbf{0.182}&0.335&0.185 &\textbf{0.330} & 0.204&	0.351 & 0.332&0.458 &	0.227&	0.387&	0.281&	0.429&	5.658&	1.671\\
&336 &\textbf{0.204}&\textbf{0.367}&0.231 &0.378 & 0.246&	0.389 & 0.655&0.670 &	0.242&	0.401&	0.293&	0.437&	4.777&	1.582\\
&720 &\textbf{0.241}&\textbf{0.396}&0.278 &0.420 & 0.268&	0.409 & 0.630&0.662 &	0.291&	0.439&	0.218&	0.387&	2.042&	1.039\\
\midrule
\multirow{4}{*}{\rotatebox{90}{$ETTm1$}}
&96 &\textbf{0.029}&\textbf{0.127}&0.033 &0.140 & 0.056&	0.183 & 0.651&0.733 &	0.109&	0.277&	0.049&	0.171&	0.296&	0.355\\
&192 &\textbf{0.041}&\textbf{0.153}&0.058 &0.186 & 0.081&	0.216 & 0.190& 0.372&	0.151&	0.310&	0.157&	0.317&	0.429&	0.474\\
&336 &\textbf{0.053}&\textbf{0.175}&0.071 &0.209 & 0.076&	0.218 & 0.428&0.581 &	0.427&	0.591&	0.289&	0.459&	0.585&	0.583\\
&720 &\textbf{0.071}&\textbf{0.205}&0.102 &0.250 & 0.110&	0.267 & 0.254&0.433 &	0.438&	0.586&	0.430&	0.579&	0.782&	0.730\\
\midrule
\multirow{4}{*}{\rotatebox{90}{$ETTm2$}} 
& 96 &0.065&\textbf{0.189}&\textbf{0.063} &0.189 & 0.065 & 0.189  & 0.153&0.318 & 0.088 & 0.225 & 0.075 & 0.208 & 0.076  &0.214   \\
& 192 &\textbf{0.094}&\textbf{0.233}& 0.102 & 0.245 & 0.118 & 0.256  &0.183 &0.350 & 0.132 &0.283 & 0.129 &0.275  & 0.132  & 0.290   \\
& 336 &\textbf{0.124}&\textbf{0.274}& 0.130 & 0.279 & 0.154 & 0.305  &0.204 &0.367  &0.180 &0.336 & 0.154 &0.302  & 0.160  & 0.312    \\
& 720 &\textbf{0.173}&\textbf{0.323}& 0.178 & 0.325 & 0.182 &0.335  &0.482 &0.567  &0.300  &0.435 & 0.160 &0.321  & 0.168  &0.335     \\
\bottomrule
\end{tabular}
}
\label{tab:uni-benchmarks-ett}
% \end{adjustwidth}
% \end{small}
\end{table*}

\section{Low-rank Approximation for FEL}
\label{app:LRA}
With the low-rank approximation of learnable matrix in Fourier Enhanced Layer significantly reducing our parameter size, here we study its effect on model accuracy on two typical datasets as shown in Table~\ref{tab:FEL_LRA}.
%\resizebox{!}{\.5\paperheight}{
\begin{table*}[h]

%\begin{wraptable}[9]{r}{0.6\textwidth}
\centering
%\begin{footnotesize}
% \begin{adjustwidth}{-1.5in}{-1in}
\caption{Low-rank Approximation (LRA) study for frequency enhanced layer: Comp. K=0 means default version without LRA, 1 means the largest compression using K=1.}
%\resizebox{\columnwidth}{!}{
\scalebox{0.75}{
\begin{tabular}{c|c|cccccccccc}
\toprule

\multicolumn{2}{c|}{Comp. K}&\multicolumn{2}{c|}{0}&\multicolumn{2}{c|}{16}&\multicolumn{2}{c|}{4}&\multicolumn{2}{c}{1}\\

\midrule
\multicolumn{2}{c|}{Metric} & MSE  & MAE & MSE & MAE& MSE  & MAE& MSE  & MAE \\
\midrule

% \multirow{4}{*}{\rotatebox{90}{$Exchange$}} 

% &96  &\textbf{0.079} &\textbf{0.204}    &0.083  &0.209  &0.082  &0.208   &0.087    &0.217     \\
% & 192  &\textbf{0.159} &\textbf{0.292}  &0.166  &0.304  &0.166  &0.304   &0.172    &0.309      \\
% & 336 & \textbf{0.270} & \textbf{0.398} &0.340  &0.436  &0.300  &0.413   &0.349    &0.452      \\
% & 720 &\textbf{0.788}& \textbf{0.680}   &1.158  &0.806  &1.147  &0.801   &0.915   &0.719      \\
\multirow{4}{*}{\rotatebox{90}{$ETTh1$}} 

&96  &\textbf{0.371} &\textbf{0.394}    &0.371  &0.397  &0.373  &0.399   & 0.391   & 0.418    \\
& 192  &0.414 &\textbf{0.423}  &0.414  &0.425  &\textbf{0.413}  &0.426   &  0.437  &  0.445    \\
& 336 & \textbf{0.442} & 0.445 &0.452  &0.451  &0.445  &\textbf{0.444}   &0.460    &0.458       \\
& 720 &\textbf{0.454}& \textbf{0.451}   &0.460  &0.472  &0.461  &0.471   &0.464    &0.476      \\

\midrule

\multirow{4}{*}{\rotatebox{90}{$Weather$}} 

&96  &\textbf{0.199} &\textbf{0.262}    &0.200  &0.266  &0.199  &0.263   &0.198    &0.261      \\
& 192  &0.228 &0.288  &0.232  &0.298  &0.227  &0.287   &\textbf{0.226}    &\textbf{0.285}       \\
& 336 & 0.267 & 0.323 &0.266  &0.320  &\textbf{0.253}  &\textbf{0.314}   &0.264    &0.316       \\
& 720 &0.319& 0.361   &\textbf{0.314}  &\textbf{0.352}  &0.319  &0.361   &0.314    &0.354      \\

\midrule
\multicolumn{2}{c|}{Parameter size}&\multicolumn{2}{c|}{100\%}&\multicolumn{2}{c|}{6.4\%}&\multicolumn{2}{c|}{1.6\%}&\multicolumn{2}{c}{0.4\%}\\
% \multirow{4}{*}{\rotatebox{90}{$Exchange$}}
% &96  &\textbf{0.079}  &\textbf{0.204}  &+15\%  & +6.8\% & +11\% & +5.2\%  & +11\%    & +5.1\% \\
% & 192 &\textbf{0.159} & \textbf{0.292} &-4.6\% & -3.8\% & +7.8\%  & +3.9\%   & +6.8\%    & +3.5\%  \\
% & 336 & \textbf{0.270}& \textbf{0.398}&-4.2\%  & -5.0\% & -3.9\%  & -6.0\%   & -7.2\%    & -8.0\% \\
% & 720 & \textbf{0.830}&\textbf{0.721} &+2.9\%  & +2.8\% & +10\%  &  +6.8\%  & +3.0\%   & +1.7\% \\
\bottomrule
\end{tabular}
\label{tab:FEL_LRA}
}
%}
% \end{adjustwidth}
%\end{footnotesize}
\end{table*}
%\end{wraptable}
%}

% \section{Proof of Theorem \ref{thm_Fourier}}

% \begin{theorem*}
% \label{thm_Fourier_correct} 
% Let $A\in\mathbbm{R}^{d\times n}$ be the Fourier coefficients matrix of an input matrix $X\in\mathbbm{R}^{d\times n}$, and $\mu(A)$, the coherence measure of matrix $A$, is $\Omega(k/n)$. We assume there exist $s$ and  a positive $ a_{\min}$ such that the elements in last $n-s$ columns of $A$ is smaller than $a_{\min}$. If we keep first $s$ columns selected and randomly choose $\mathcal{O}(k^2/\epsilon^2 - s)$ columns from the remaining parts, with high probability
% \[
%     \|A - P(A)\|_F \leq \mathcal{O}\left[(1 + \epsilon)a_{\min}\cdot\sqrt{(n-s)d}\right],
% \]
% where  $P(A)$ denotes the matrix projecting $A$ onto the column selected column space.
% \end{theorem*}
% (In Theorem \ref{thm_Fourier_correct}, we correct a typo error in Theorem \ref{thm_Fourier}. The ``in last d - s columns...'' should be ``in last n - s columns...''). 

% \begin{proof}
% Similar to the analysis in Appendix C of~\cite{FedFormer}, let $A_k = P(A)$ and $A_{\bar{k}}$ be the matrix projecting A onto the remaining-column space, where the columns are not selected. $A = A_k + A_{\bar{k}}$. So we have $\|A - P(A)\|_F = \| A_{\bar{k}}\|$. In the assumption of Theorem \ref{thm_Fourier_correct}, the elements in $A_{\bar{k}}$ is smaller than $a_{\min}$, thus $\| A_{\bar{k}}\|_F = \sqrt{\mathrm{trace}(A_{\bar{k}}^\top \cdot A_{\bar{k}})} \leq a_{\min} \cdot \sqrt{(n-s)d}$. ($A_{\bar{k}} \in \mathbb{R}^{d \times (n-s)}$)
% \end{proof}
% % In we observe that 

\section{Theoretical Analysis}

\subsection{Theorem 1}
The proof is a simple extension of Proposition 6 in \cite{Hippo}. We omit it for brevity.

\subsection{Theorem 2}
% In order to generate a stable sequence $\{x_t\}$, we restrict the matrix $A$ to be unitary. The above Theorem indicates that the uncertain portion between $x_{t}$  and its estimation $A^{\theta}x_{t-\theta} + \sum_{i=1}^{\theta-1}A^{i}b$ at time $t-\theta$ is scaled with $\sqrt{\theta}$. The larger $\theta$ will lead to higher uncertainty and it in turn leads less correlation between $x_t$ and $x_{t-\theta}$. Therefore introducing more historical information may not necessary lead better performance.
As we have $x_t = Ax_{t-1} + b - \epsilon_{t-1}$ for $t=2,3,...\theta$, we recursively use them and the following result holds:
\begin{align}
    x_{t} &= Ax_{t-1} +  b + \epsilon_{t-1}\notag\\
    &= A(Ax_{t-2} +  b + \epsilon_{t-2})+  b + \epsilon_{t-1}\notag\\
    &=A^2x_{t-2} + Ab + b + A\epsilon_{t-2} + \epsilon_{t-1}\notag\\
    % &=A^3x_{t-3} +  A^2b  + Ab + b + A^2\epsilon_{t-3}+ A\epsilon_{t-2} + \epsilon_{t-1}\notag\\
    &\cdots\notag\\
    &=A^{\theta}x_{t-\theta} + \sum_{i=1}^{\theta-1}A^ib+ \underbrace{\sum_{i=1}^{\theta-1}A^i\epsilon_{t-i}}_{(*)}\notag.
\end{align}
Following Hoeffding inequality, for $\mu>0$ we have
\begin{align}
    \mathbbm{P}\left(|(*)|\ge \mu\right)\le \exp\left(-\frac{2\mu^2}{\sum_{i=1}^{\theta -1}\|A^i\epsilon_{t-1}\|_{\psi_2}^2}\right),
\end{align}
where $\|\cdot\|_{\psi_2}$ is the Orlicz norm defined as
\begin{align}
    \|X\|_{\psi_2} :=\inf\left\{c\ge 0: \mathbbm{E}[\exp(X^2/c^2)]\le 2\right\}\notag.
\end{align}
Since we require $A$ being unitary, we will have $\|A\epsilon\|_2^2 = \|\epsilon\|_2^2$ and it implies $\|A^i\epsilon_{t-1}\|_{\psi_2}^2\| = \|\epsilon_{t-1}\|_{\psi_2}^2 =   \mathcal{O}(\sigma^2)$ for $i=1,2,...,\theta$. The desirable result follows by setting $\mu = \mathcal{O}(\sqrt{\theta}\sigma)$.

\subsection{Theorem 3}

% \begin{theorem*}
% \label{thm_Fourier_correct} 
% Let $A\in\mathbbm{R}^{d\times n}$ be the Fourier coefficients matrix of an input matrix $X\in\mathbbm{R}^{d\times n}$, and $\mu(A)$, the coherence measure of matrix $A$, is $\Omega(k/n)$. We assume there exist $s$ and  a positive $ a_{\min}$ such that the elements in last $n-s$ columns of $A$ is smaller than $a_{\min}$. If we keep first $s$ columns selected and randomly choose $\mathcal{O}(k^2/\epsilon^2 - s)$ columns from the remaining parts, with high probability
% \[
%     \|A - P(A)\|_F \leq \mathcal{O}\left[(1 + \epsilon)a_{\min}\cdot\sqrt{(n-s)d}\right],
% \]
% where $P(A)$ denotes the matrix projecting $A$ onto the column selected column space.
% \end{theorem*}
% (In Theorem \ref{thm_Fourier_correct}, we correct a typo error in Theorem \ref{thm_Fourier}. The ``in last d - s columns...'' should be ``in last n - s columns...''). 

% \begin{proof}
As we keep first $s$ columns selected, $P(A)-A$ has all $0$ elements in first $s$ columns. We thus ignore them and consider the approximation quality on $\tilde{A}\in\mathbb{R}^{d\times (n-s)}$ with the sampled columns.  Via the similar analysis in Appendix C of \cite{FedFormer}, with high probability we have $\| \tilde{A}-P(A) \|_F \leq (1+\epsilon) \|\tilde{A} - \tilde{A}_k\|_F$, where $\tilde{A}_k$ is the ``best” rank-$k$ approximation provided by truncating the singular value decomposition (SVD) of $\tilde{A}$, and where $\|\cdot\|_F$
is the Frobenius norm. As we assume the element in last $n - s$ columns of $A$ is smaller than $a_{\min}$, one can verify  $\| \tilde{A}-P(A) \|_F\le \sqrt{d \times (n-s)}a_{\min}$ and desirable result follows immediately.  
% \end{proof}

% \input{appendix/mode_selection}
\section{Parameter Sensitivity}
\label{app:parameter}
\paragraph{Influence of Legendre Polynomial number $N$ and Frequency mode number $M$}
\begin{figure*}[h]
    \centering
    \includegraphics[width=0.8\linewidth]{figures/MSE_vs_N/N_vs_dataset_all_15.eps}
    \caption{The reconstruction error (MSE) vs. Legendre Polynomial number ($N$) on three datasets with three different input lengths.}
    \label{fig:MSE_vs_Hippo_N}
\end{figure*}
The experimental results on three different datasets (ETTm1, Electricity, and Exchange) in Figure \ref{fig:MSE_vs_Hippo_N} show the optimal choice of Legendre Polynomials number ($N$) when we aim to minimize the reconstruction error (in MSE) on the historical data. The MSE error decreases sharply at first and saturates at an optimal point, where $N$ is in proportion to the input length. For input sequences with lengths of 192, 336, and 720, $N$ $\approx$ 40, 60, and 100 gives the minimal MSE,  respectively. %We select a default N = 256 to give our model enough representation powder for a long term historical signal recover with multiscale mechanism implemented.

\begin{figure*}[h]
    \centering
    % \includegraphics{figures/MSE_vs_N/elc_192.eps}
    % (a)
    \includegraphics[width=0.99\linewidth]{figures/N_vs_modes/N_vs_modes_all_ecl.eps}
    % (b)
    % \includegraphics[width=0.28\linewidth]{figures/N_vs_modes/N_vs_modes_pr336_ecl.eps}
    % (c)
    % \includegraphics[width=0.28\linewidth]{figures/N_vs_modes/N_vs_modes_pr720_ecl.eps}
    \caption{The MSE error of univariate time series forecasting task on Electricity dataset with different Legendre Polynomials number ($N$), mode number and input length. Left: input length = 192. Mid: input length = 336. Right: input length = 720.}
    \label{fig:MSE_vs_modes_vs_N}
\end{figure*}

Figure \ref{fig:MSE_vs_modes_vs_N} shows the MSE error of time series forecasting on the Electricity dataset, with different Legendre Polynomials number ($N$), mode number, and input length. We observe that, when enlarging $N$, the model performance saturates at an optimal point. For example, in Figure \ref{fig:MSE_vs_modes_vs_N} Left (input length=192), the best performance is reached when $N>64$. While in Figure \ref{fig:MSE_vs_modes_vs_N} Right (input length=720), the best performance is reached when $N$ is larger than 128. Another influential parameter is the mode number. From Figure \ref{fig:MSE_vs_modes_vs_N} we observe that a small mode number will lead to better performance, as a module with a small mode number works as a denoising filter.
\section{Noise Injection Experiment}
\label{app:noise}
Our model's robustness in long-term forecasting tasks can be demonstrated using a series of noise injection experiments as shown in Table \ref{tab:ablation_noise}. As we can see, adding Gaussian noise in the training/test stage has a limited effect on our model's performance, since the %average 
deterioration is less than 1.5\% in the worst case. The model's robustness is consistent across various forecasting horizons. Note that adding the noise in the testing stage other than the training stage will even improve our performance by 0.4\%, which further supports our claim of robustness. 
%\resizebox{!}{\.5\paperheight}{
\begin{table*}[h]
\centering
%\begin{footnotesize}
% \begin{adjustwidth}{-1.5in}{-1in}
\caption{Noise injection studies. A 0.3*$\mathcal{N}\left(0,1\right)$ Gaussian noise is introduced into our training/testing. We conduct 4 sets of experiments with/without noise in training and test phases. The experiments are performed on ETTm1 and Electricity with different output lengths. The metric of variants is presented in relative value ('+' indicates degraded performance, and '-' indicates improved performance).}
%\resizebox{\columnwidth}{!}{
\scalebox{0.75}{
\begin{tabular}{c|c|cccccccc}
\toprule

\multicolumn{2}{c|}{Training}&\multicolumn{4}{c|}{noise}&\multicolumn{4}{c}{with noise}\\
\midrule
\multicolumn{2}{c|}{Testing}&\multicolumn{2}{c|}{without noise}&\multicolumn{2}{c|}{with noise}&\multicolumn{2}{c|}{without noise}&\multicolumn{2}{c}{with noise}\\

\midrule
\multicolumn{2}{c|}{Metric} & MSE  & MAE & MSE & MAE& MSE  & MAE& MSE  & MAE \\
\midrule
% \multirow{4}{*}{\rotatebox{90}{$ETTm2$}} &96 & \textbf{0.165} & \textbf{0.256} &0.203 &0.287 &0.255  &0.339 &0.705 &0.690 &0.365  &0.453  &0.768  &0.642  &0.658  &0.619    \\
%                         & 192 & \textbf{0.240} & \textbf{0.313} &0.269  &0.328  &0.281 &0.340 &0.924 &0.692 &0.533  &0.563  &0.989  &0.757  &1.078  &0.827    \\
%                         & 336 & \textbf{0.286} & \textbf{0.345} & 0.325 &0.366 &0.339  &0.372 &1.364 &0.877 &1.363&0.887  &1.334  &0.872  &1.549  &0.972     \\
%                         & 720 & \textbf{0.393} & \textbf{0.410} &0.421 &0.415 &0.422  &0.419 &0.877 &1.074 &3.379  &1.338 & 3.048 &1.328  &2.631  &1.242      \\
% \midrule
\multirow{4}{*}{\rotatebox{90}{$ETTh1$}} 

&96  &\textbf{0.371} &\textbf{0.394}    &-1.6\%  & -2.0\% & -0.0\% & -0.0\%  & -1.6\%   & -2.0\%     \\
& 192  &\textbf{0.414} &\textbf{0.423}  &-0.5\%  & -1.4\%    & +0.5\% & -0.0\%  & -0.5\%   & -1.4\%    \\
& 336 & \textbf{0.442} & \textbf{0.445} &-1.8\% & -0.9\%    & -0.9\% & +1.3\%  & -3.2\%   & -1.6\%     \\
& 720 &\textbf{0.465}& \textbf{0.472}   &+0.2\%     & -0.2\%     &+0.9\%    & +0.9\%  & -0.6\%    & -0.4\%    \\

% \midrule

% \multirow{4}{*}{\rotatebox{90}{$Exchange$}}
% &96  &\textbf{0.079}  &\textbf{0.204}  &+15\%  & +6.8\% & +11\% & +5.2\%  & +11\%    & +5.1\% \\
% & 192 &\textbf{0.159} & \textbf{0.292} &-4.6\% & -3.8\% & +7.8\%  & +3.9\%   & +6.8\%    & +3.5\%  \\
% & 336 & \textbf{0.270}& \textbf{0.398}&-4.2\%  & -5.0\% & -3.9\%  & -6.0\%   & -7.2\%    & -8.0\% \\
% & 720 & \textbf{0.830}&\textbf{0.721} &+2.9\%  & +2.8\% & +10\%  &  +6.8\%  & +3.0\%   & +1.7\% \\
\bottomrule
\end{tabular}
\label{tab:ablation_noise}
}
%}
% \end{adjustwidth}
%\end{footnotesize}
\end{table*}
%}
\section{Distribution Analysis of Forecasting Output}
\label{app:Distribution}
\subsection{Kolmogorov-Smirnov Test}
We adopt the Kolmogorov-Smirnov (KS) test to check whether our model's input and output sequences come from the same distribution. The KS test is a nonparametric test for checking the equality of probability distributions. In essence, the test answers the following question ``Are these two sets of samples drawn from the same distribution?''. 
The Kolmogorov-Smirnov statistic is defined as:
$$
D_{n, m}=\sup _{x}\left|F_{1, n}(x)-F_{2, m}(x)\right|, 
$$
where $\sup$ is the supremum function, $F_{1, n}$ and $F_{2, m}$ are the empirical distribution functions of the two compared samples.
For samples that are large enough, the null hypothesis would be rejected at level $\alpha$ if
$$
D_{n, m}>\sqrt{-\frac{1}{2}\ln \left(\frac{\alpha}{2}\right)} \cdot \sqrt{\frac{n+m}{n \cdot m}},
$$
where $n$ and $m$ are the first and second sample sizes.
\subsection{Distribution Analysis}
In this section, we evaluate the distribution similarity between models' input and output sequences using the KS test. In Table \ref{tab:KStest_small}, we applied the Kolmogrov-Smirnov test to check if the output sequences of various models that trained on ETTm1/ETTm2 are consistent with the input sequence. 
%This method is better used on some stationary time series datasets such as electric load forecast. 
On both datasets, by setting the standard P-value as 0.01, various existing baseline models have much smaller P-values except FEDformer and Autoformer, which indicates their outputs have a high probability of being sampled from different distributions compared to their input signals. Autoformer and FEDformer have much larger P-values mainly due to their seasonal-trend decomposition mechanism. The proposed FiLM also has a much larger P-value compared to most baseline models. And its null hypothesis can not be rejected in most cases for these two datasets. It implies that the output sequence generated by FiLM shares a similar pattern as the input signal, and thus justifies our design motivation of FiLM as discussed in Section~\ref{sec_intro}. Though FiLM gets a smaller P-value than FEDformer, it is close to the actual output, which indicates that FiLM makes a good balance between recovering and forecasting. 

\begin{table}[h]
%\setlength{\uppercaptionskip}{0.pt}
%\setlength{\belowcaptionskip}{-0.pt}
%\vskip 0.15in
\centering
\caption{P-values of Kolmogrov-Smirnov test of different Transformer models for long-term forecasting output on ETTm1 and ETTm2 dataset. Larger value indicates the hypothesis (the input sequence and forecasting output come from the same distribution) is less likely to be rejected. The largest results are highlighted.}
\begin{small}
% \begin{sc}
\vskip 0.05in
\scalebox{0.80}{
\begin{tabular}{c|c|cccccc}
\toprule
\multicolumn{2}{c|}{Methods}&Transformer&Informer&Autoformer&FEDformer&FiLM&True\\ %&\multicolumn{2}{c|}{Fedformer-f }\\%&\multicolumn{2}{c|}{}&\\
\midrule
\multirow{4}{*}{\rotatebox{90}{ETTm1}} 
& 96 & 0.0090 & 0.0055&0.020 & \textbf{0.048} & 0.016& {0.023} \\
& 192 & 0.0052 & 0.0029&0.015 & \textbf{0.028} & 0.0123& {0.013} \\
& 336 & 0.0022 & 0.0019&0.012 & \textbf{0.015} & 0.0046& {0.010} \\
% & 720 & 0.0023 & 0.0016 & \textbf{0.014} & \textbf{0.0036} \\
& 720 & 0.0023 & 0.0016&0.008 & \textbf{0.014} & 0.0024& {0.004} \\
\midrule
\multirow{4}{*}{\rotatebox{90}{ETTm2}} 
% & 48 & 0.454 & & 0.366 & & 0.476 & & 0.356 \\
& 96 & 0.0012 & 0.0008& \textbf{0.079} &{0.071} & 0.022 & {0.087} \\%& \textbf{0.379} & \textbf{0.419}\\
& 192 & 0.0011 & 0.0006& \textbf{0.047} &{0.045}  &0.020 & {0.060} \\%& \textbf{0.426} & \textbf{0.441}\\
% & 288 & 0.634 & & 0.430 & & 0.571 & & 0.379 \\
& 336 & 0.0005 & 0.00009& 0.027 &\textbf{0.028} &0.012 & {0.042} \\%& \textbf{0.445} & \textbf{0.459}\\
% & 672 & 0.606 & & 0.528 & & 0.544 & & 0.501\\
& 720 & 0.0008& 0.0002& \textbf{0.023} & {0.021} &0.0081 & {0.023} \\
% \multicolumn{2}{c|}{Count}& 0 & 0 & 3 & 5 & 7& NA \\
%& \textbf{0.543} & \textbf{0.490}\\
%& -96 & 0.0012 & 0.0009 & 0.0001 & 0.0037 & \textbf{0.039} & \textbf{0.012} \\
\bottomrule
\end{tabular}
}
\label{tab:KStest_small}
% \end{sc}
\end{small}
%\end{center}
\vskip -0.1in
\end{table}

\section{Learnable Parameter Size}
\label{app:sec:learnable_para_size}

Compared to Transformer-based baseline models, FiLM enjoys a lightweight property with \textbf{80\%} learnable parameter reduction as shown in Table \ref{tab:size}. It has the potential to be used in mobile devices, or, in some situations where a lightweight model is preferred.

\begin{table}[h]
\centering
\caption{Parameter size of baseline models and FiLM with different low-rank approximations: the models are trained and tested on ETT dataset; the subscript number denotes $k$ in low-rank approximation.}
\begin{small}
% \begin{sc}
\vskip 0.05in
\begin{tabular}{c|ccccccc}
\toprule
Methods&Transformer&Autoformer&FEDformer&FiLM&$\mathrm{FiLM}_{16}$ & $\mathrm{FiLM}_4$ & $\mathrm{FiLM}_1$\\
\midrule
Parameter(M) & 0.0069 & 0.0069& 0.0098& 1.50 & 0.0293 &0.0062& 0.00149 \\
%&\multicolumn{2}{c|}{Fedformer-f }\\%&\multicolumn{2}{c|}{}&\\
\bottomrule
\end{tabular}
\label{tab:size}
% \end{sc}
\end{small}
%\end{center}
\vskip -0.1in
\end{table}

\section{Training Speed and Memory Usage}
\label{app:time}

\begin{figure*}[h]
    \centering
    % \includegraphics{figures/MSE_vs_N/elc_192.eps}
    % (a)
    \includegraphics[width=0.45\linewidth]{figures/speed_memory/model_memory_hippo.eps}
    \includegraphics[width=0.45\linewidth]{figures/speed_memory/model_speed_hippo.eps}
    % (b)
    % \includegraphics[width=0.28\linewidth]{figures/N_vs_modes/N_vs_modes_pr336_ecl.eps}
    % (c)
    % \includegraphics[width=0.28\linewidth]{figures/N_vs_modes/N_vs_modes_pr720_ecl.eps}
    \caption{(Left) the memory usage of FiLM and baseline models. (Right) training speed of FiLM and baseline models. The input length is fixed to 96 and the output length is 768, 1536, 3072, 4608, and 7680.}
    \label{fig:Mem_Time}
\end{figure*}

\begin{figure*}[h]
    \centering
    % \includegraphics{figures/MSE_vs_N/elc_192.eps}
    % (a)
    \includegraphics[width=0.7\linewidth]{figures/speed_memory/model_speed_score_scatter_nhits.eps}
    % \includegraphics[width=0.45\linewidth]{figures/speed_memory/model_speed_hippo.eps}
    % (b)
    % \includegraphics[width=0.28\linewidth]{figures/N_vs_modes/N_vs_modes_pr336_ecl.eps}
    % (c)
    % \includegraphics[width=0.28\linewidth]{figures/N_vs_modes/N_vs_modes_pr720_ecl.eps}
    \caption{Comparison of training speed and performance of benchmarks. The experiment is performed on ETTm2 with output length = 96, 192, 336, and 720. The performance of the models is measured with \textit{Score}, where $Score=1/MSE$. The radius of the circle measured the STD of the performance. A higher \textit{Score} indicates better performance, same for \textit{Speed}. A smaller circle indicates better robustness. The \textit{Speed} and \textit{Score} are presented on relative value.}
    \label{fig:Time_score_scatter}
\end{figure*}

\paragraph{Memory Usage}
As shown in Figure \ref{fig:Mem_Time} (Left), FiLM has good memory usage with the prolonging output length. For a fair comparison, we fix the experimental settings of \textit{Xformer}, where we fix the input length as 96 and prolong the output length. From Figure \ref{fig:Mem_Time} (Left), we can observe that FiLM has a quasi-constant memory usage. Note that the memory usage of FiLM is only linear to the input length. Furthermore, FiLM enjoys a much smaller memory usage than others because of the simple architecture and compressed parameters with low-rank approximation as discussed in Appendix~\ref{app:sec:learnable_para_size}.

\paragraph{Training Speed}
Experiments are performed on one NVIDIA V100 32GB GPU. As shown in Figure \ref{fig:Mem_Time} (Right), FiLM has a faster training speed than others with the prolonging output length. For a fair comparison, we fix the experimental setting of \textit{Xformer}, where we fix the input length as 96 and prolong the output length. However, in the real experiment settings, we use a longer input length (much longer than 96). Thus, the experiment in Figure \ref{fig:Mem_Time} (Right) is merely a toy case to show the tendency. In Figure \ref{fig:Time_score_scatter}, we show the average epoch time vs average performance under the settings of benchmarks. The experiment is performed on ETTm2 dataset with output lengths = 96, 192, 336, and 720. Because of the extremely low memory usage of FiLM, it can be trained with a larger batch size (batch size = 256) on only one GPU compared with baselines (batch size = 32). In Figure \ref{fig:Time_score_scatter}, FiLM-256 is the FiLM models trained with batch size = 256, it exhibits significant advantages on both speed and accuracy. Furthermore, due to the shallow structure and smaller amount of trainable parameters, FiLM is easy to converge and enjoys smaller performance variation and smaller performance degradation when using a large batch size. It is observed that the models with Fourier enhanced block (FiLM \& FEDformer) have better robustness. It is also worth noting that the vanilla Transformer has good training speed because of the not-so-long sequence length. Only a sequence length over one thousand will distinguish the advantage of efficient Transformers.

% high because of a heavy projection step and its resulting large intermediate tensor. A efficient FiLM model is one of our future work. 

%\input{appendix/theoretical_analysis}

\section{Additional Benchmarks}
\subsection{Multivariate long-term series forecasting with extra baseline models}
For the additional benchmarks for multivariate experiments, we add some non-Transformer methods for comparison.N-BEATS\cite{nbeats} and N-HiTS\cite{challu2022n} are two recent proposed powerful non-Transformer methods. As N-HiTS is the latest development from the research group, which also published N-BEATS, we add N-HiTS to our empirical comparison. Here, we adopt the results in the N-HiTS paper to prevent inappropriate parameter tuning problems. We also add a seasonal-naive model in the comparison. FiLM outperforms N-HiTS in most cases(33/48). Moreover, Simple Seasonal-naive\cite{seasonal-naive} is a solid baseline on exchange datasets better than N-hits, Fedformer, and Autoformer, but FiLM still surpasses its performance, as shown in Table \ref{tab:multi-benchmarks}.
%\resizebox{!}{\.5\paperheight}{
% \vskip -0.2in
\begin{table*}[h!]
\centering
%\begin{footnotesize}
% \begin{adjustwidth}{-1.5in}{-1in}
\caption{multivariate long-term series forecasting results on six datasets with various input length and prediction length $O \in \{96,192,336,720\}$ (For ILI dataset, we set prediction length $O \in \{24,36,48,60\}$). Supplementary results of non-Transformer baselines (N-Hits and a seasonal-naive model).}
% \vspace{-1mm}
\scalebox{0.8}{
\begin{tabular}{c|c|cccccccccccccccc|}
\toprule
\multicolumn{2}{c|}{Methods}&\multicolumn{2}{c|}{FiLM}&\multicolumn{2}{c|}{N-Hits}&\multicolumn{2}{c|}{FEDformer}&\multicolumn{2}{c|}{Autoformer}&\multicolumn{2}{c|}{Seasonal-naive}\\
\midrule
\multicolumn{2}{c|}{Metric} & MSE  & MAE & MSE & MAE& MSE  & MAE& MSE  & MAE& MSE  & MAE \\
\midrule
\multirow{4}{*}{\rotatebox{90}{$ETTm2$}} 
                        &96 & \textbf{0.165} & 0.256 & 0.176 & \textbf{0.255} &0.203 &0.287 &0.255  &0.339  &0.262 &0.300 \\
                        & 192 & \textbf{0.222} & \textbf{0.296} & 0.245 & 0.305 & 0.269  &0.328  &0.281 &0.340  &0.319 &0.337\\
                        & 336 & \textbf{0.277} & \textbf{0.333} & 0.295 & 0.346 & 0.325 &0.366 &0.339  &0.372  &0.375 &0.371\\
                        & 720 & \textbf{0.371} & \textbf{0.389} & 0.401 & 0.426 & 0.421 &0.415 &0.422  &0.419 &0.469 &0.422\\
\midrule
\multirow{4}{*}{\rotatebox{90}{$Electricity$}} 
                        &96  &0.154  &0.267 & \textbf{0.147} & \textbf{0.249}  &0.183 &0.297 &0.201  &0.317 &0.211 &0.278\\
                        & 192 &\textbf{0.164} & \textbf{0.258} & 0.167 & 0.269 & 0.195 &0.308 &0.222  &0.334 &0.214 &0.282\\
                        & 336 & 0.188 & \textbf{0.283} & \textbf{0.186} & 0.290 & 0.212 &0.313 &0.231 &0.338 &0.226 &0.294\\
                        & 720 & 0.236 & \textbf{0.332} & 0.243 & 0.340 &\textbf{0.231} &0.343 &0.254  &0.361 &0.265 & 0.324\\
\midrule
\multirow{4}{*}{\rotatebox{90}{$Exchange$}} 
                        &96  & \textbf{0.086} & \textbf{0.204} &0.092 & 0.211 & 0.139 & 0.276 & 0.197 &0.323 &0.086 &0.204 \\
                        & 192 & \textbf{0.189} & \textbf{0.292} & 0.208 & 0.322 &0.256 &0.369 & 0.300 & 0.369 &0.172 &0.295\\
                        & 336 & \textbf{0.356} & \textbf{0.433} & 0.371 & 0.443 & 0.426 &0.464 & 0.509 & 0.524 &0.311 &0.401\\
                        & 720 & \textbf{0.727} & \textbf{0.669} & 0.888 & 0.723 &  1.090 &0.800 & 1.447 & 0.941 &0.832 &0.686\\
\midrule
\multirow{4}{*}{\rotatebox{90}{$Traffic$}} 
                        &96  & 0.416& 0.294 & \textbf{0.402} & \textbf{0.282} & 0.562 &0.349 &0.613  &0.388 &1.219 &0.497\\
                        & 192 & \textbf{0.408} & \textbf{0.288} &0.420 & 0.297 & 0.562 &0.346 &0.616&0.382 &1.089 &0.456\\
                        & 336 & \textbf{0.425} & \textbf{0.298} &0.448 & 0.313 & 0.570 &0.323 &0.622  &0.337 &1.147 &0.473\\
                        & 720 & \textbf{0.520} &\textbf{0.353} &0.539 & 0.353 & 0.596 &0.368 &0.660  &0.408 &1.181 &0.486\\
\midrule
\multirow{4}{*}{\rotatebox{90}{$Weather$}} 
                        & 96 & 0.199 & 0.262 & \textbf{0.158} & \textbf{0.195} & 0.217  &0.296  &0.266  &0.336 &0.315 &0.288\\
                        & 192 & 0.228 & 0.288 & \textbf{0.211} & \textbf{0.247} & 0.276  &0.336  &0.307  &0.367 &0.341 &0.305\\
                        & 336 &\textbf{0.267} & 0.323 & 0.274 & \textbf{0.300} & 0.339  &0.380  &0.359  &0.395 &0.381 &0.331\\
                        & 720 &\textbf{0.319} & 0.361 &0.351 & \textbf{0.353} & 0.403  &0.428 &0.578 &0.578 &0.440 &0.370 \\
\midrule
\multirow{4}{*}{\rotatebox{90}{$ILI$}} 
                        & 24 & 1.970 & 0.875 & \textbf{1.862} & \textbf{0.869} & 2.203  &0.963  &3.483 &1.287 &6.581 &1.699 \\
                        & 36 & \textbf{1.982} & \textbf{0.859} &2.071 & 0.969 & 2.272  &0.976  &3.103  &1.148 &7.121 &1.882 \\
                        & 48 & \textbf{1.868} & \textbf{0.896} &2.346 & 1.042 & 2.209  &0.981  &2.669  &1.085 &6.567 &1.797 \\
                        & 60 & \textbf{2.057} & \textbf{0.929} &2.560 & 1.073 & 2.545  &1.061  &2.770  &1.125 &5.885 &1.675 \\
\bottomrule
\end{tabular}
\label{tab:multi-benchmarks}
}
% \end{adjustwidth}
%\end{footnotesize}
\end{table*}
\subsection{Ablation univariate forecasting experiments for FEL layers with all six datasets }
As shown in Table \ref{tab:ablation_FEL_full}, although LPU+MLP combining all boosting tricks has slightly better performance than FiLM for the ETTm1 dataset, FiLM remains the most consistent and effective model among all variants across all six datasets. FEL is a much better backbone structure than MLP, LSTM, CNN, and vanilla attention modules. 

%\resizebox{!}{\.5\paperheight}{
\begin{table*}[!h]
\vskip -0.05in
\centering
%\begin{footnotesize}
% \begin{adjustwidth}{-1.5in}{-1in}
\caption{: (Full Benchmark)Ablation studies of FEL layer. The FEL layer is replaced with 4 different variants: MLP, LSTM, CNN, and Transformer.The experiments are performed on ETTm1 and Electricity. The metric of variants is presented in relative value (’+’ indicates degraded performance, ’-’ indicates improved performance).}\vspace{-1mm}
\scalebox{0.8}{
\begin{tabular}{c|c|ccccccccccccccc}
\toprule
\multicolumn{2}{c|}{Methods}&\multicolumn{2}{c|}{FilM}&\multicolumn{2}{c|}{LPU+MLP}&\multicolumn{2}{c|}{LPU+LSTM}&\multicolumn{2}{c|}{LPU+CNN}&\multicolumn{2}{c|}{LPU+attention}\\
\midrule
\multicolumn{2}{c|}{Metric} & MSE  & MAE & MSE & MAE& MSE  & MAE& MSE  & MAE& MSE  & MAE& \\
\midrule

\multirow{4}{*}{\rotatebox{90}{ETTm1}} 

&96  &\textbf{0.029} &\textbf{0.127}  &+0.0\%   & +0.0\%   & +12.1\% & +7.1\%    & +13.5\%   & +9.5\%   & +1.7\%  & +1.6\%  \\
& 192  &\textbf{0.041} &\textbf{0.153}  &-1.5\% & -0.6\%  & +12.2\% & +8.5\%  & +10.8\%   & +7.8\%    & +2.0\%  & +3.3\%  \\
& 336 & \textbf{0.053} & \textbf{0.175} &-1.7\% & -1.7\%  & +4.5\% & +4.0\%    & +10.8\%    & +6.3\%    & +4.5\% & +2.9\%   \\
& 720 &\textbf{0.071}& \textbf{0.205}   &-0.9\%  & -1.0\%  & +5.5\% & +3.4\%  & +8.6\%    & +4.9\%    & +13.8\% & +7.8\%   \\

\midrule
\multirow{4}{*}{\rotatebox{90}{Electricity}} 

&96  &\textbf{0.154}  &\textbf{0.247}  &+155\%  & +81\%   & +160\% & +84\%    & +330\%  & +155\%  & +242\% & +119\%  \\%&--& -- & \\
& 192 &\textbf{0.166} & \textbf{0.258} &+59\% & +39\%   & +121\%  & +67\%   & +224\%  & +117\%  & +264\% & +131\%  \\%&--& --  \\
& 336 & \textbf{0.188}& \textbf{0.283} &+55\%  & +35\%   & +150\%  & +74\%   & +128\%  & +71\% & +183\% & +95\%  \\%&--& -- \\
& 720 & \textbf{0.249}&\textbf{0.341}  &+33\%  & +25\%   & +154\%  & +73\%   & +192\%  & +95\%  & +312\% & +138\%  \\ %&--& --  \\

\midrule
\multirow{4}{*}{\rotatebox{90}{Exchange}} 

&96  &\textbf{0.110}  &\textbf{0.247}  &-13\%  & -12\%   & +51\% & +17\%    & +4.6\%  & -1.2\%  & -4.6\% & -5.8\%  \\%&--& -- & \\
& 192 &\textbf{0.207} & \textbf{0.352} &+7.2\% & +0.0\%   & +69\%  & +32\%   & +29\%  & +12\%  & +22\% & +11\%  \\%&--& --  \\
& 336 & \textbf{0.327}& \textbf{0.461} &+48\%  & +13\%   & +62\%  & +20\%   & +68\%  & +24\% & +72\% & +23\%  \\%&--& -- \\
& 720 & \textbf{0.811}&\textbf{0.708}  &+29\%  & +14\%   & +24\%  & +9.6\%   & +38\%  & +12\%  & +64\% & +27\%  \\ %&--& --  \\

\midrule
\multirow{4}{*}{\rotatebox{90}{Traffic}} 

&96  &\textbf{0.144}  &\textbf{0.215}  &+69\%  & +47\%   & +13\% & +15\%    & +300\%  & +176\%  & +271\% & +161\%  \\%&--& -- & \\
& 192 &\textbf{0.120} & \textbf{0.199} &+17\% & +7.5\%   & +31\%  & +24\%   & +258\%  & +149\%  & +1572\% & +355\%  \\%&--& --  \\
& 336 & \textbf{0.128}& \textbf{0.212} &+6.2\%  & +7.6\%   & +16\%  & +15\%   & +151\%  & +102\% & +1514\% & +368\%  \\%&--& -- \\
& 720 & \textbf{0.153}&\textbf{0.252}  &+38\%  & +28\%   & +11\%  & +7.9\%   & +250\%  & +126\%  & +1048\% & +349\%  \\ %&--& --  \\

\midrule
\multirow{4}{*}{\rotatebox{90}{Weather}} 

&96  &\textbf{0.0012}  &\textbf{0.026}  &+17\%  & +6.2\%   & +16\% & +6.9\%    & +19\%  & +8.1\%  & +21\% & +8.9\%  \\%&--& -- & \\
& 192 &\textbf{0.0014} & \textbf{0.029} &-1.4\% & -2.4\%   & +5.0\%  & +1.7\%   & 0.7\%  & -0.7\%  & +4.3\% & +1.4\%  \\%&--& --  \\
& 336 & \textbf{0.0015}& \textbf{0.030} &+0.0\%  & -0.6\%   & +3.3\%  & +1.3\%   & +2.0\%  & +0.0\% & +3.3\% & +1.3\%  \\%&--& -- \\
& 720 & \textbf{0.0022}&\textbf{0.037}  &+4.6\%  & -0.3\%   & +4.1\%  & -1.6\%   & 3.6\%  & 0.0\%  & +0.0\% & -3.8\%  \\ %&--& --  \\

\midrule
\multirow{4}{*}{\rotatebox{90}{ILI}} 

&96  &\textbf{0.629}  &\textbf{0.538}  &+51\%  & +45\%   & -2.5\% & 9.5\%    & +20\%  & +29\%  & +112\% & +59\%  \\%&--& -- & \\
& 192 &\textbf{0.444} & \textbf{0.481} &+99\% & +58\%   & +25\%  & +24\%   & +84\%  & +56\%  & +360\% & +142\%  \\%&--& --  \\
& 336 & \textbf{0.557}& \textbf{0.584} &+33\%  & +31\%   & +21\%  & +16\%   & +58\%  & +30\% & +702\% & +94\%  \\%&--& -- \\
& 720 & \textbf{0.641}&\textbf{0.644}  &+8.4\%  & +5.4\%   & +23\%  & +18\%   & +42\%  & +22\%  & +74\% & +34\%  \\ %&--& --  \\
\bottomrule
\end{tabular}
\label{tab:ablation_FEL_full}
}
% \end{adjustwidth}
%\end{footnotesize}

\vskip -0.05in
\end{table*}
%}

\subsection{Boosting experiments of LPU with common deep learning backbones for all six datasets}
As shown in Table \ref{tab:boosting}, LPU shows a consistent boosting effect across all selected common deep learning backbones for most datasets. It can be used as a simple and effective build add-on block for long-term time series forecasting tasks. Although without data normalization, pure LPU negatively boosts performance for some cases. 

%\resizebox{!}{\.5\paperheight}{
\vskip -0.1in
% \begin{wraptable}

%\begin{wraptable}[12]{r}{0.7\textwidth}
\begin{table*}[h]
\centering
%\begin{footnotesize}
% \begin{adjustwidth}{-1.5in}{-1in}
\caption{(Full Benchmark) Boosting effect of LPU layer for common deep learning backbones: MLP, LSTM, CNN and Attention.`+` indicates degraded performance.}\vspace{-1mm}
\scalebox{0.80}{
\begin{tabular}{c|c|cccccccccccccccccc}
%\begin{tabular}{c|c|cccccccccc}
\toprule
\multicolumn{2}{c|}{Methods}&\multicolumn{2}{c|}{FEL}&\multicolumn{2}{c|}{MLP}&\multicolumn{2}{c|}{LSTM}&\multicolumn{2}{c|}{lagged-LSTM}&\multicolumn{2}{c|}{CNN}&\multicolumn{2}{c}{Attention}\\
\midrule
% \multicolumn{2}{c|}{Metric} & MSE  & MAE & MSE & MAE& MSE  & MAE& MSE  & MAE& MSE  & MAE& MSE  & MAE&\\
\multicolumn{2}{c|}{Compare} & LPU  & Linear& LPU  & Linear & LPU  & Linear & LPU  & Linear & LPU  & Linear & LPU  & Linear\\
\midrule

\multirow{4}{*}{\rotatebox{90}{ETTm1}} 

&96  &\textbf{0.030}  & +38\%   & 0.034  & +8.0\%  & 0.049 & +73\% & 0.093 & -21\% & 0.116   & -50\%   & 0.243  & -81\% \\
& 192  &\textbf{0.047} & +9.5\% & 0.049  & +30\%  & 0.174 & +32\% & 0.331 & -48\% & 0.101   & +20\%    & 0.387  & -86\% \\
& 336 & 0.063 & +5.8\% & \textbf{0.061}  & +64\%  & 0.119 & +84\% & 0.214 & -19\% & 0.122   & +25\%    & 1.652  & +12\% \\
& 720 &\textbf{0.081} & +1.4\%  & 0.082  & +62\%  & 0.184 & +32\% & 0.303 & -6.5\%  & 0.108   & +13\%    & 4.782  & -61\% \\

\midrule
\multirow{4}{*}{\rotatebox{90}{Electricity}} 

&96  &\textbf{0.213}  & +136\%  & 0.431  & +121\%   & 0.291 & +56\% & 0.739 & -33\% & 0.310  & +43\%  & 0.805 & +23\% \\%&--& --
& 192 &\textbf{0.268} & +32\%   & 0.291 & +239\%   & 0.353  & +17\% & 0.535 & +15\% & 0.380  & +12\%  & 0.938 & +14\% \\%&--& --  \\
& 336 & 0.307& +0.1\%  & \textbf{0.296} & +235\%   & 0.436  & -6.7\% & 0.517 & +23\% & 0.359  & +29\% & 2.043 & -54\% & \\%&--& -- \\
& 720 & \textbf{0.321}& +37\%   & 0.339 & +196\%   & 0.636  & -11\% & 0.492 & +28\% & 0.424  & +18\%  & 9.115 & +298\% \\ %&--& --  \\
               
\midrule
\multirow{4}{*}{\rotatebox{90}{$Exchange$}} 
& 96  & 0.130 & +7.5\% & \textbf{0.110} & -18\% & 0.224 & +6.0\% & 0.521 & -58\% & 0.244 & -18\% & 0.338 & +872\% \\
& 192 & \textbf{0.205} & +39\% & 0.257 & -36\% & 0.787 & -35\% & 1.742 & -66\% & 0.630 & +2.1\% & 0.930 & +278\% \\
& 336 & 0.467 & +9.2\% & \textbf{0.461} & -33\% & 0.964 & +24\% & 2.281 & -38\% & 3.231 & -85\% & 1.067 & +69\%\\
& 720 & \textbf{1.003} & +26\% & 1.981 & -61\% & 2.703 & -29\% & 1.457 & +34\% & 5.531 & +9.7\% & 0.631 & +1831\% \\
\midrule

\multirow{4}{*}{\rotatebox{90}{$Traffic$}} 
&96  &\textbf{0.312} & +18\% & 0.376 & +277\% & 0.215 & +1.2\% & 0.216 & +10\% & 0.543 & -33\% & 0.429 & +210\% \\
& 192 & \textbf{0.141} & +9.6\% & 0.199 & +598\% & 0.177 & +19\% & 0.186 & +17\% & 0.451 & +9.0\% & 0.476 & +176\% \\
& 336 & \textbf{0.143} & +2.5\% & 0.195 & +613\% & 0.192 & +19\% & 0.190 & +11\% & 0.346 & +44\% & 0.377 & +260\% \\
& 720 & \textbf{0.215} & +30\% & 0.240 & +475\% & 0.234 & -1.7\% & 0.250 & +15\% & 0.348 &  +47\% & 0.773 & +171\%\\
\midrule

\multirow{4}{*}{\rotatebox{90}{$Weather$}} 
& 96 & 0.0073 & -38\% & 0.006  & -33\% & 0.006 & -23\% & 0.0070 & -17\% & \textbf{0.0022} & +167\% & 0.0065 &-11\%\\
& 192 & 0.0106 & -64\% & 0.007 & -14\% & 0.0074 & -11\% & \textbf{0.0063} & -19\% & 0.007 & -24\% & 0.0075 & -12\%\\
& 336 & 0.0079 & -37\% & 0.006 & +4.9\% & 0.0056 & +12\% & \textbf{0.0055} & +12\% & 0.0056 & +0.5\% & 0.222 & -69\% \\
& 720 &0.0063 & +0.4\% & 0.006 & +7.6\% & \textbf{0.0062} & +5.3\% & 0.103 & -36\% &0.006 & +4.2\% & 0.037 & -81\% \\
                        
\midrule
\multirow{4}{*}{\rotatebox{90}{$ILI$}} 
& 24 & 1.393 &	+6.1\% & \textbf{1.220} & +36\% & 2.306 & +66\% & 4.189 & -9.2\% & 2.264 & -22\% & 2.249 & +217\% \\
& 36 & 1.242 & -22\% & \textbf{1.185} & +56\% & 2.950 & +44\% & 2.516 & +42\% & 1.841 & -3.0\% & 5.026 & +45\% \\
& 48 & 1.448 & -28\% & \textbf{1.079} & +79\% & 3.385 & +38\% & 3.501 & +16\% & 1.654 & +23\% & 2.838 & +115\% \\
& 60 & 2.089 & -18\% & \textbf{0.986} & +96\%  & 4.031 & +18\% & 4.258 & +10\% & 1.290 & +176\% & 4.978 & +250\% \\
\bottomrule
\end{tabular}
\label{tab:boosting}
}
% \end{adjustwidth}
%\end{footnotesize}
\end{table*}
%\end{wraptable}
%}

\subsection{Ablation univariate forecasting experiments for Low rank approximation with all six datasets}
As shown in Table \ref{tab:FEL_LRA_FULL}, with the low-rank approximation of learnable matrix in the Fourier Enhanced Layer significantly reduces our parameter size, and even improves our model's performance for some datasets.
%\resizebox{!}{\.5\paperheight}{
\begin{table*}[h]

%\begin{wraptable}[9]{r}{0.6\textwidth}
\centering
%\begin{footnotesize}
% \begin{adjustwidth}{-1.5in}{-1in}
\caption{Low-rank Approximation (LRA) univariate forecasting study for frequency enhanced layer: Comp. K=0 means default version without LRA, 1 means the largest compression using K=1.}
%\resizebox{\columnwidth}{!}{
\scalebox{0.75}{
\begin{tabular}{c|c|cccccccccc}
\toprule

\multicolumn{2}{c|}{Comp. K}&\multicolumn{2}{c|}{0}&\multicolumn{2}{c|}{16}&\multicolumn{2}{c|}{4}&\multicolumn{2}{c}{1}\\

\midrule
\multicolumn{2}{c|}{Metric} & MSE  & MAE & MSE & MAE& MSE  & MAE& MSE  & MAE \\
\midrule

% \multirow{4}{*}{\rotatebox{90}{$Exchange$}} 

% &96  &\textbf{0.079} &\textbf{0.204}    &0.083  &0.209  &0.082  &0.208   &0.087    &0.217     \\
% & 192  &\textbf{0.159} &\textbf{0.292}  &0.166  &0.304  &0.166  &0.304   &0.172    &0.309      \\
% & 336 & \textbf{0.270} & \textbf{0.398} &0.340  &0.436  &0.300  &0.413   &0.349    &0.452      \\
% & 720 &\textbf{0.788}& \textbf{0.680}   &1.158  &0.806  &1.147  &0.801   &0.915   &0.719      \\
\multirow{4}{*}{\rotatebox{90}{$ETTm2$}} 

&96&0.065&0.189&0.064&0.185&\textbf{0.064}&\textbf{0.185}&0.064&0.186 \\

&192&0.094&0.233&0.094&0.231&0.093&0.231&\textbf{0.093}&\textbf{0.231} \\

&336&0.124&0.274&0.124&0.270&\textbf{0.124}&\textbf{0.269}&0.124&0.271 \\

&720&0.173&0.323&0.173&0.322&\textbf{0.173}&\textbf{0.322}&0.177&0.328 \\
\midrule

\multirow{4}{*}{\rotatebox{90}{$Electricity$}} 

&96&\textbf{0.154}&\textbf{0.247}&0.211&0.324&0.216&0.331&0.277&0.387 \\

&192&\textbf{0.166}&\textbf{0.258}&0.251&0.352&0.246&0.347&0.334&0.421 \\

&336&\textbf{0.188}&\textbf{0.283}&0.276&0.369&0.302&0.396&0.363&0.440 \\

&720&\textbf{0.249}&\textbf{0.341}&0.336&0.429&0.342&0.436&0.411&0.481 \\

\midrule

\multirow{4}{*}{\rotatebox{90}{$Exchange$}} 

&96&0.110&0.259&0.119&0.273&\textbf{0.104}&\textbf{0.247}&0.105&0.251 \\

&192&0.207&0.352&0.196&0.355&\textbf{0.195}&\textbf{0.349}&0.212&0.372 \\

&336&\textbf{0.327}&\textbf{0.461}&0.388&0.497&0.373&0.491&0.407&0.506 \\

&720&\textbf{0.811}&\textbf{0.708}&0.908&0.767&1.288&0.941&1.840&1.153 \\
\midrule

\multirow{4}{*}{\rotatebox{90}{$Traffic$}} 

&96&\textbf{0.144}&\textbf{0.215}&0.146&0.223&0.154&0.237&0.267&0.373 \\

&192&\textbf{0.120}&\textbf{0.199}&0.121&0.201&0.138&0.231&0.218&0.333 \\

&336&0.128&0.212&\textbf{0.120}&\textbf{0.206}&0.132&0.227&0.216&0.335 \\

&720&\textbf{0.153}&\textbf{0.252}&0.155&0.257&0.154&0.257&0.246&0.366 \\

\midrule

\multirow{4}{*}{\rotatebox{90}{$Weather$}} 

&96&0.0012&0.026&0.0011&0.025&\textbf{0.001}&\textbf{0.025}&0.001&0.025 \\

&192&0.0014&0.029&0.0014&0.028&\textbf{0.001}&\textbf{0.028}&0.001&0.028 \\

&336&0.0015&0.03&0.0015&0.030&\textbf{0.001}&\textbf{0.029}&0.002&0.030 \\

&720&0.0022&0.037&0.0022&0.037&\textbf{0.002}&\textbf{0.037}&0.002&0.037 \\
\midrule

\multirow{4}{*}{\rotatebox{90}{$ILI$}} 

&96&0.629&0.538&\textbf{0.599}&\textbf{0.556}&0.628&0.558&0.630&0.579 \\

&192&\textbf{0.444}&\textbf{0.481}&0.487&0.533&0.508&0.561&0.570&0.612 \\

&336&0.557&0.584&\textbf{0.553}&\textbf{0.565}&0.703&0.696&0.722&0.706 \\

&720&\textbf{0.641}&\textbf{0.644}&0.648&0.641&0.900&0.780&1.493&1.032 \\

\midrule
\multicolumn{2}{c|}{Parameter size}&\multicolumn{2}{c|}{100\%}&\multicolumn{2}{c|}{6.4\%}&\multicolumn{2}{c|}{1.6\%}&\multicolumn{2}{c}{0.4\%}\\
% \multirow{4}{*}{\rotatebox{90}{$Exchange$}}
% &96  &\textbf{0.079}  &\textbf{0.204}  &+15\%  & +6.8\% & +11\% & +5.2\%  & +11\%    & +5.1\% \\
% & 192 &\textbf{0.159} & \textbf{0.292} &-4.6\% & -3.8\% & +7.8\%  & +3.9\%   & +6.8\%    & +3.5\%  \\
% & 336 & \textbf{0.270}& \textbf{0.398}&-4.2\%  & -5.0\% & -3.9\%  & -6.0\%   & -7.2\%    & -8.0\% \\
% & 720 & \textbf{0.830}&\textbf{0.721} &+2.9\%  & +2.8\% & +10\%  &  +6.8\%  & +3.0\%   & +1.7\% \\
\bottomrule
\end{tabular}
\label{tab:FEL_LRA_FULL}
}
%}
% \end{adjustwidth}
%\end{footnotesize}
\end{table*}
%\end{wraptable}
%}

\subsection{Ablation univariate forecasting experiments for frequency mode selection with all six datasets}
Three different mode selection policies are studied for frequency enhanced layer: 1) lowest mode selection: we select $m$ lowest frequency modes to retain. 2) random model selection: we select $m$ frequency modes randomly to retain. 3) lowest with extra high mode selection: we select $0.8\times m$ lowest frequency modes and $0.2\times m$ high-frequency modes randomly to retain. The experimental results are summarized in Table \ref{tab:mode_full} with $m = 64$ for both experiments. The lowest mode selection is the most stable frequency mode selection policy through adding some randomness mode can improve the results for some datasets.

% \begin{wraptable}[16]{r}{0.6\textwidth}
\begin{table*}[h]

% \begin{wraptable}[11]{r}{0.5\textwidth}
\vskip -0.1in

\centering
\caption{Mode selection policy study for frequency enhanced layer. Lowest: select the lowest $m$ frequency mode; Random: select $m$ random frequency mode; Low random: select the $0.8*m$ lowest frequency mode and $0.2*m$ random high frequency mode.}\vspace{-1.5mm}
\scalebox{0.75}{
\begin{tabular}{c|c|cccccccc}
\toprule
\multicolumn{2}{c|}{Policy}&\multicolumn{2}{c|}{Lowest}&\multicolumn{2}{c|}{Random}&\multicolumn{2}{c}{Low random}\\
\midrule
\multicolumn{2}{c|}{Metric} & MSE  & MAE & MSE & MAE& MSE  & MAE \\
\midrule
\multirow{4}{*}{\rotatebox{90}{ETTm2}} 
&96&\textbf{0.065}&\textbf{0.189}&0.066&0.189&0.066&0.190 \\

&192&\textbf{0.094}&\textbf{0.233}&0.096&0.235&0.096&0.235 \\

&336&\textbf{0.124}&0.274&0.125&\textbf{0.270}&0.128&0.275 \\

&720&0.173&0.323&\textbf{0.173}&\textbf{0.322}&0.173&0.323 \\

\midrule
\multirow{4}{*}{\rotatebox{90}{Electricity}} 
&96&\textbf{0.154}&\textbf{0.247}&0.175&0.0.260&0.176&0.262 \\

&192&\textbf{0.166}&\textbf{0.258}&0.177&0.266&0.168&0.273 \\

&336&\textbf{0.188}&\textbf{0.283}&0.199&0.289&0.192&0.299 \\

&720&\textbf{0.249}&\textbf{0.341}&0.269&0.364&0.270&0.362 \\

\midrule
\multirow{4}{*}{\rotatebox{90}{Exchange}} 
&96&0.11&0.259&0.110&0.256&\textbf{0.106}&\textbf{0.249} \\

&192&0.207&0.352&\textbf{0.196}&\textbf{0.351}&0.207&0.357 \\

&336&\textbf{0.327}&\textbf{0.461}&0.451&0.522&0.373&0.484 \\

&720&0.811&0.708&0.835&0.714&\textbf{0.604}&\textbf{0.628} \\

\midrule
\multirow{4}{*}{\rotatebox{90}{Traffic}} 
&96&\textbf{0.144}&\textbf{0.215}&0.145&0.216&0.145&0.217 \\

&192&0.12&0.199&0.119&0.198&\textbf{0.118}&\textbf{0.197} \\

&336&0.128&0.212&\textbf{0.122}&\textbf{0.207}&0.122&0.209 \\

&720&0.153&0.252&\textbf{0.142}&\textbf{0.238}&0.155&0.259 \\

\midrule
\multirow{4}{*}{\rotatebox{90}{Weather}} 
&96&\textbf{0.0012}&\textbf{0.026}&0.0012&0.027&0.0012&0.026 \\

&192&\textbf{0.0014}&\textbf{0.029}&0.0014&0.029&0.0014&0.029 \\

&336&\textbf{0.0015}&\textbf{0.03}&0.0015&0.030&0.0015&0.030 \\

&720&\textbf{0.0022}&\textbf{0.037}&0.0023&0.037&0.0023&0.037 \\

\midrule
\multirow{4}{*}{\rotatebox{90}{ILI}} 
&96&0.629&0.538&0.639&0.542&\textbf{0.626}&\textbf{0.537} \\

&192&\textbf{0.444}&\textbf{0.481}&0.448&0.490&0.447&0.494 \\

&336&\textbf{0.557}&\textbf{0.584}&0.560&0.590&0.557&0.587 \\

&720&\textbf{0.641}&\textbf{0.644}&0.641&0.647&0.643&0.650 \\

\bottomrule

\end{tabular}
\label{tab:mode_full}
}
\end{table*}
% \end{wraptable}
