# Supplementary material for: GCformer: An Efficient Framework for Accurate and Scalable Long-Term Multivariate Time Series Forecasting
Source: arXiv:2306.08325 source file (2023-08-15)
Supplement: Supplementary file 2 [file 0_appendix_main.tex]

\section{Visualization}

\begin{figure*}[t]
\centering
% \scalebox{0.70}{
\includegraphics[width=0.95\linewidth]{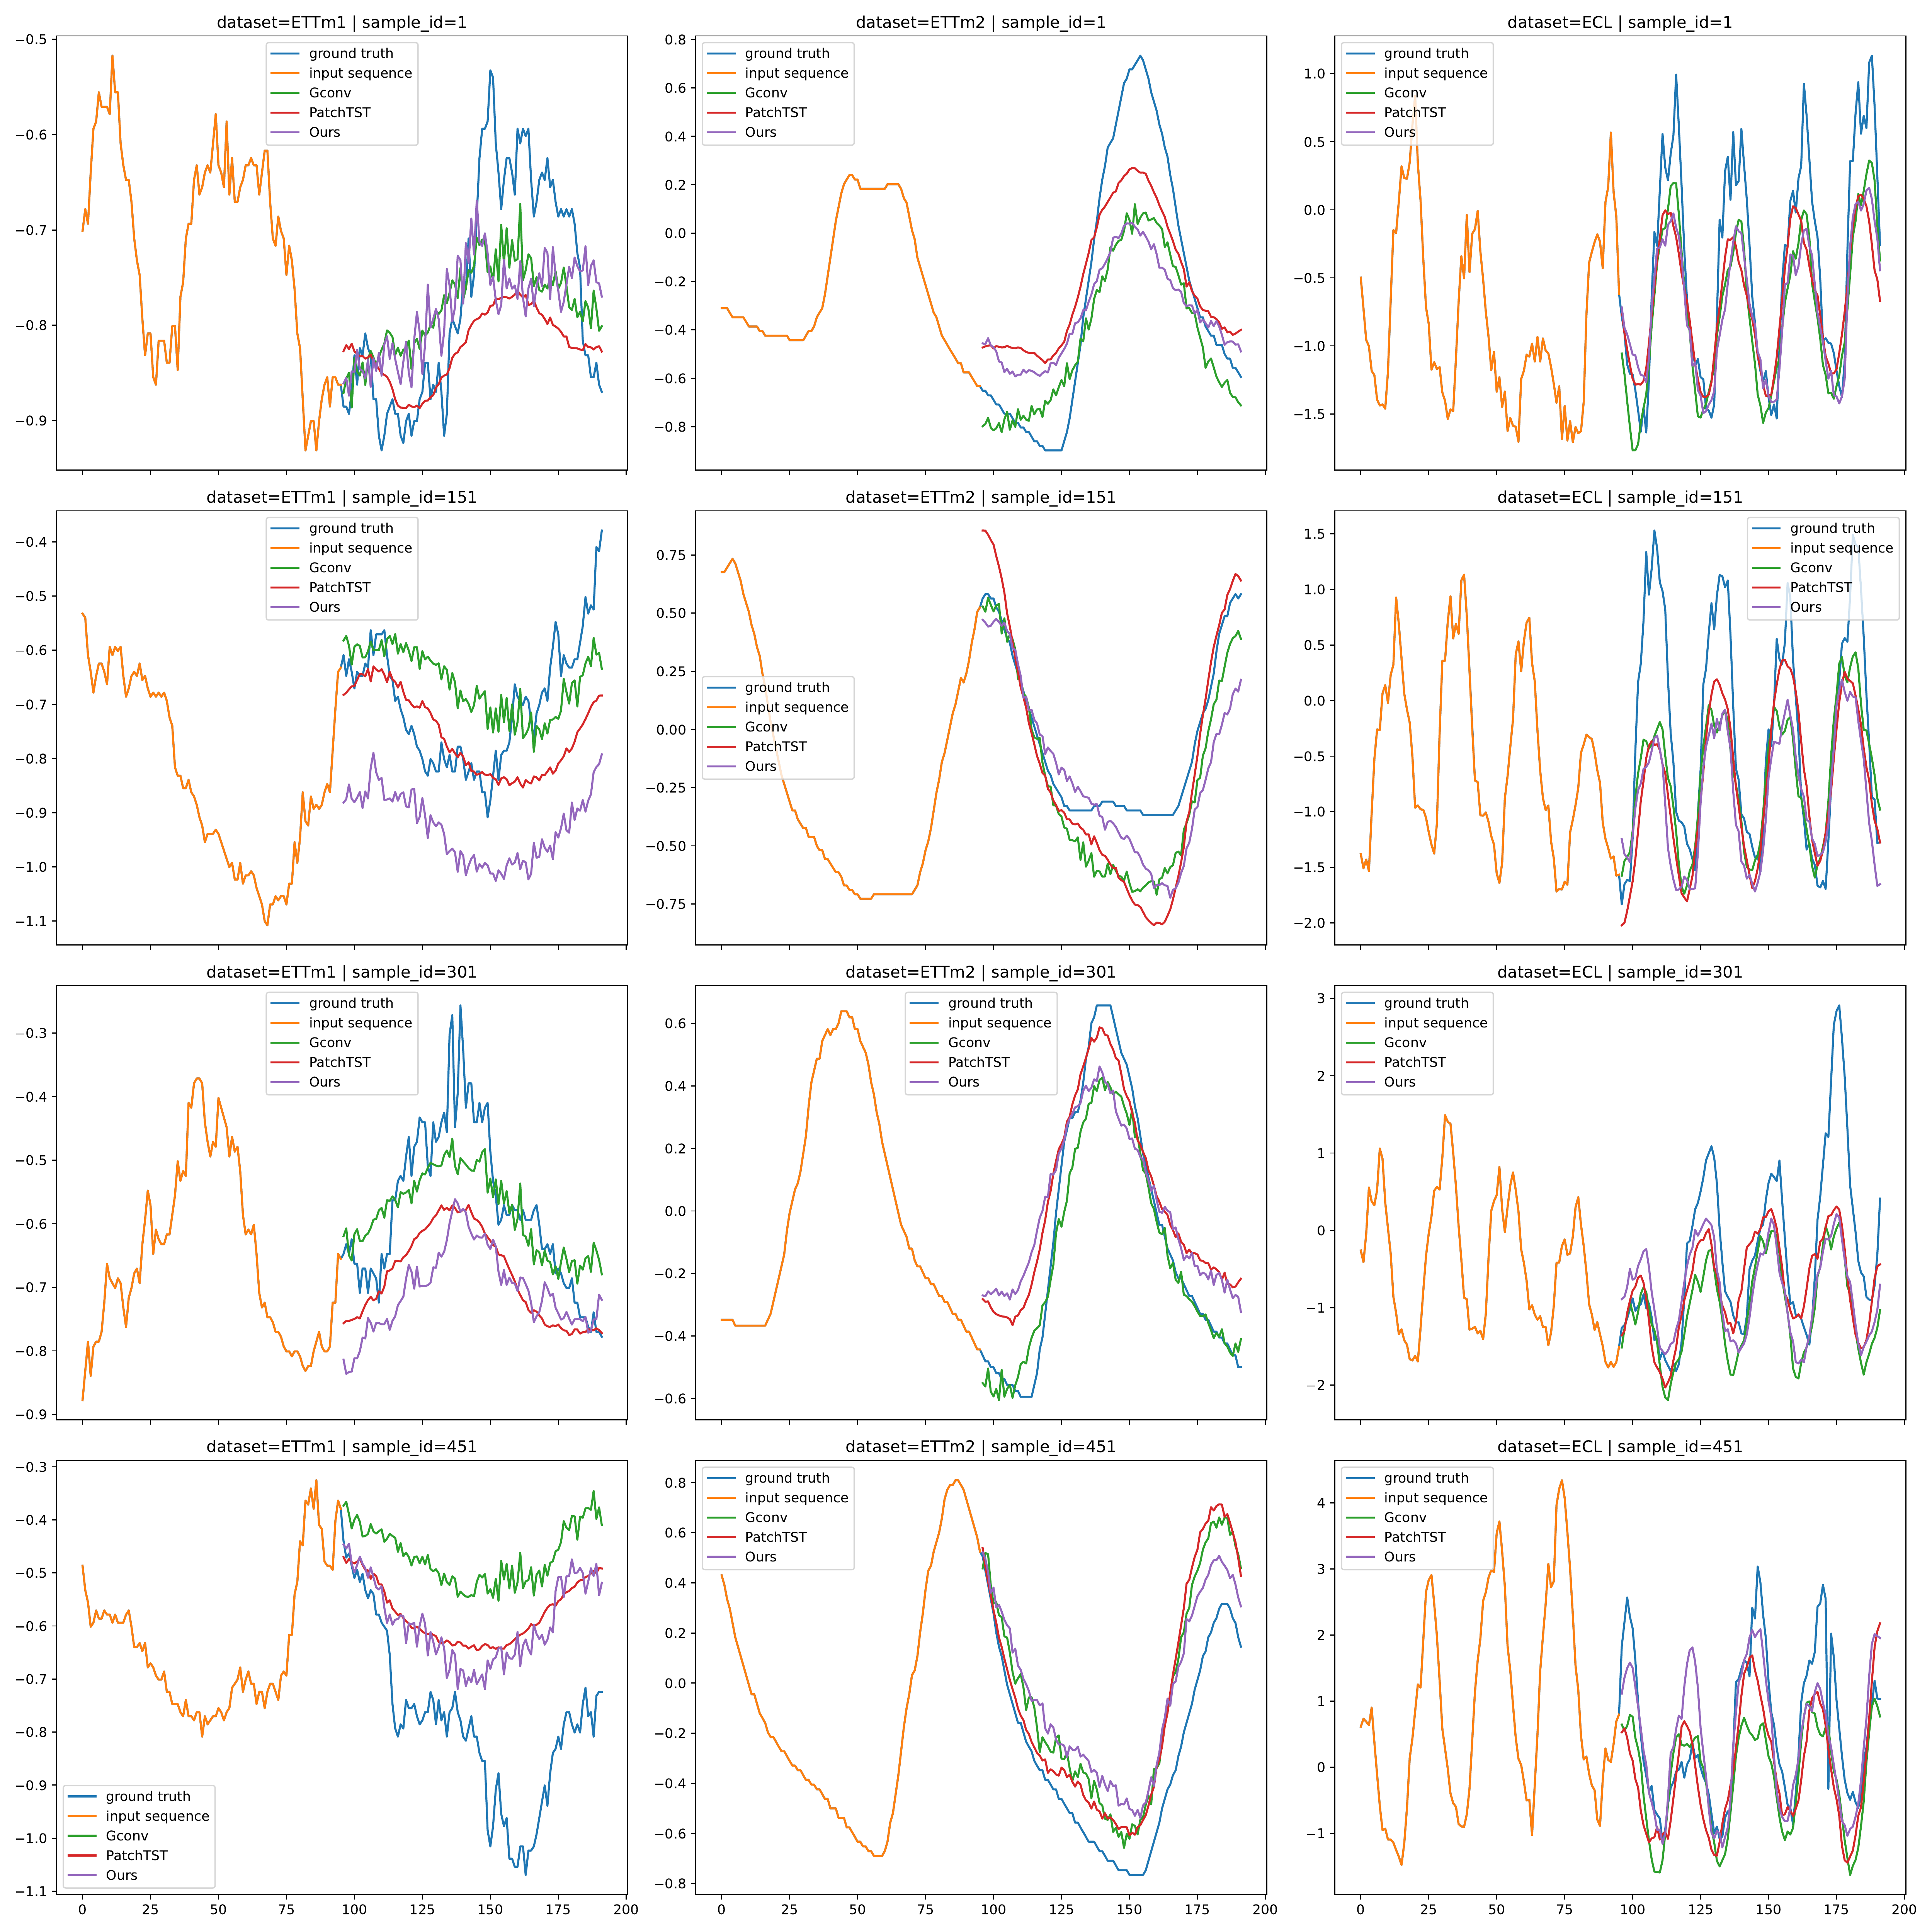}
\caption{Visualization of 96 step forecasting }
\label{fig:boost}
% \vskip -0.2in
\end{figure*}

\begin{figure*}[t]
\centering
% \scalebox{0.70}{
\includegraphics[width=0.95\linewidth]{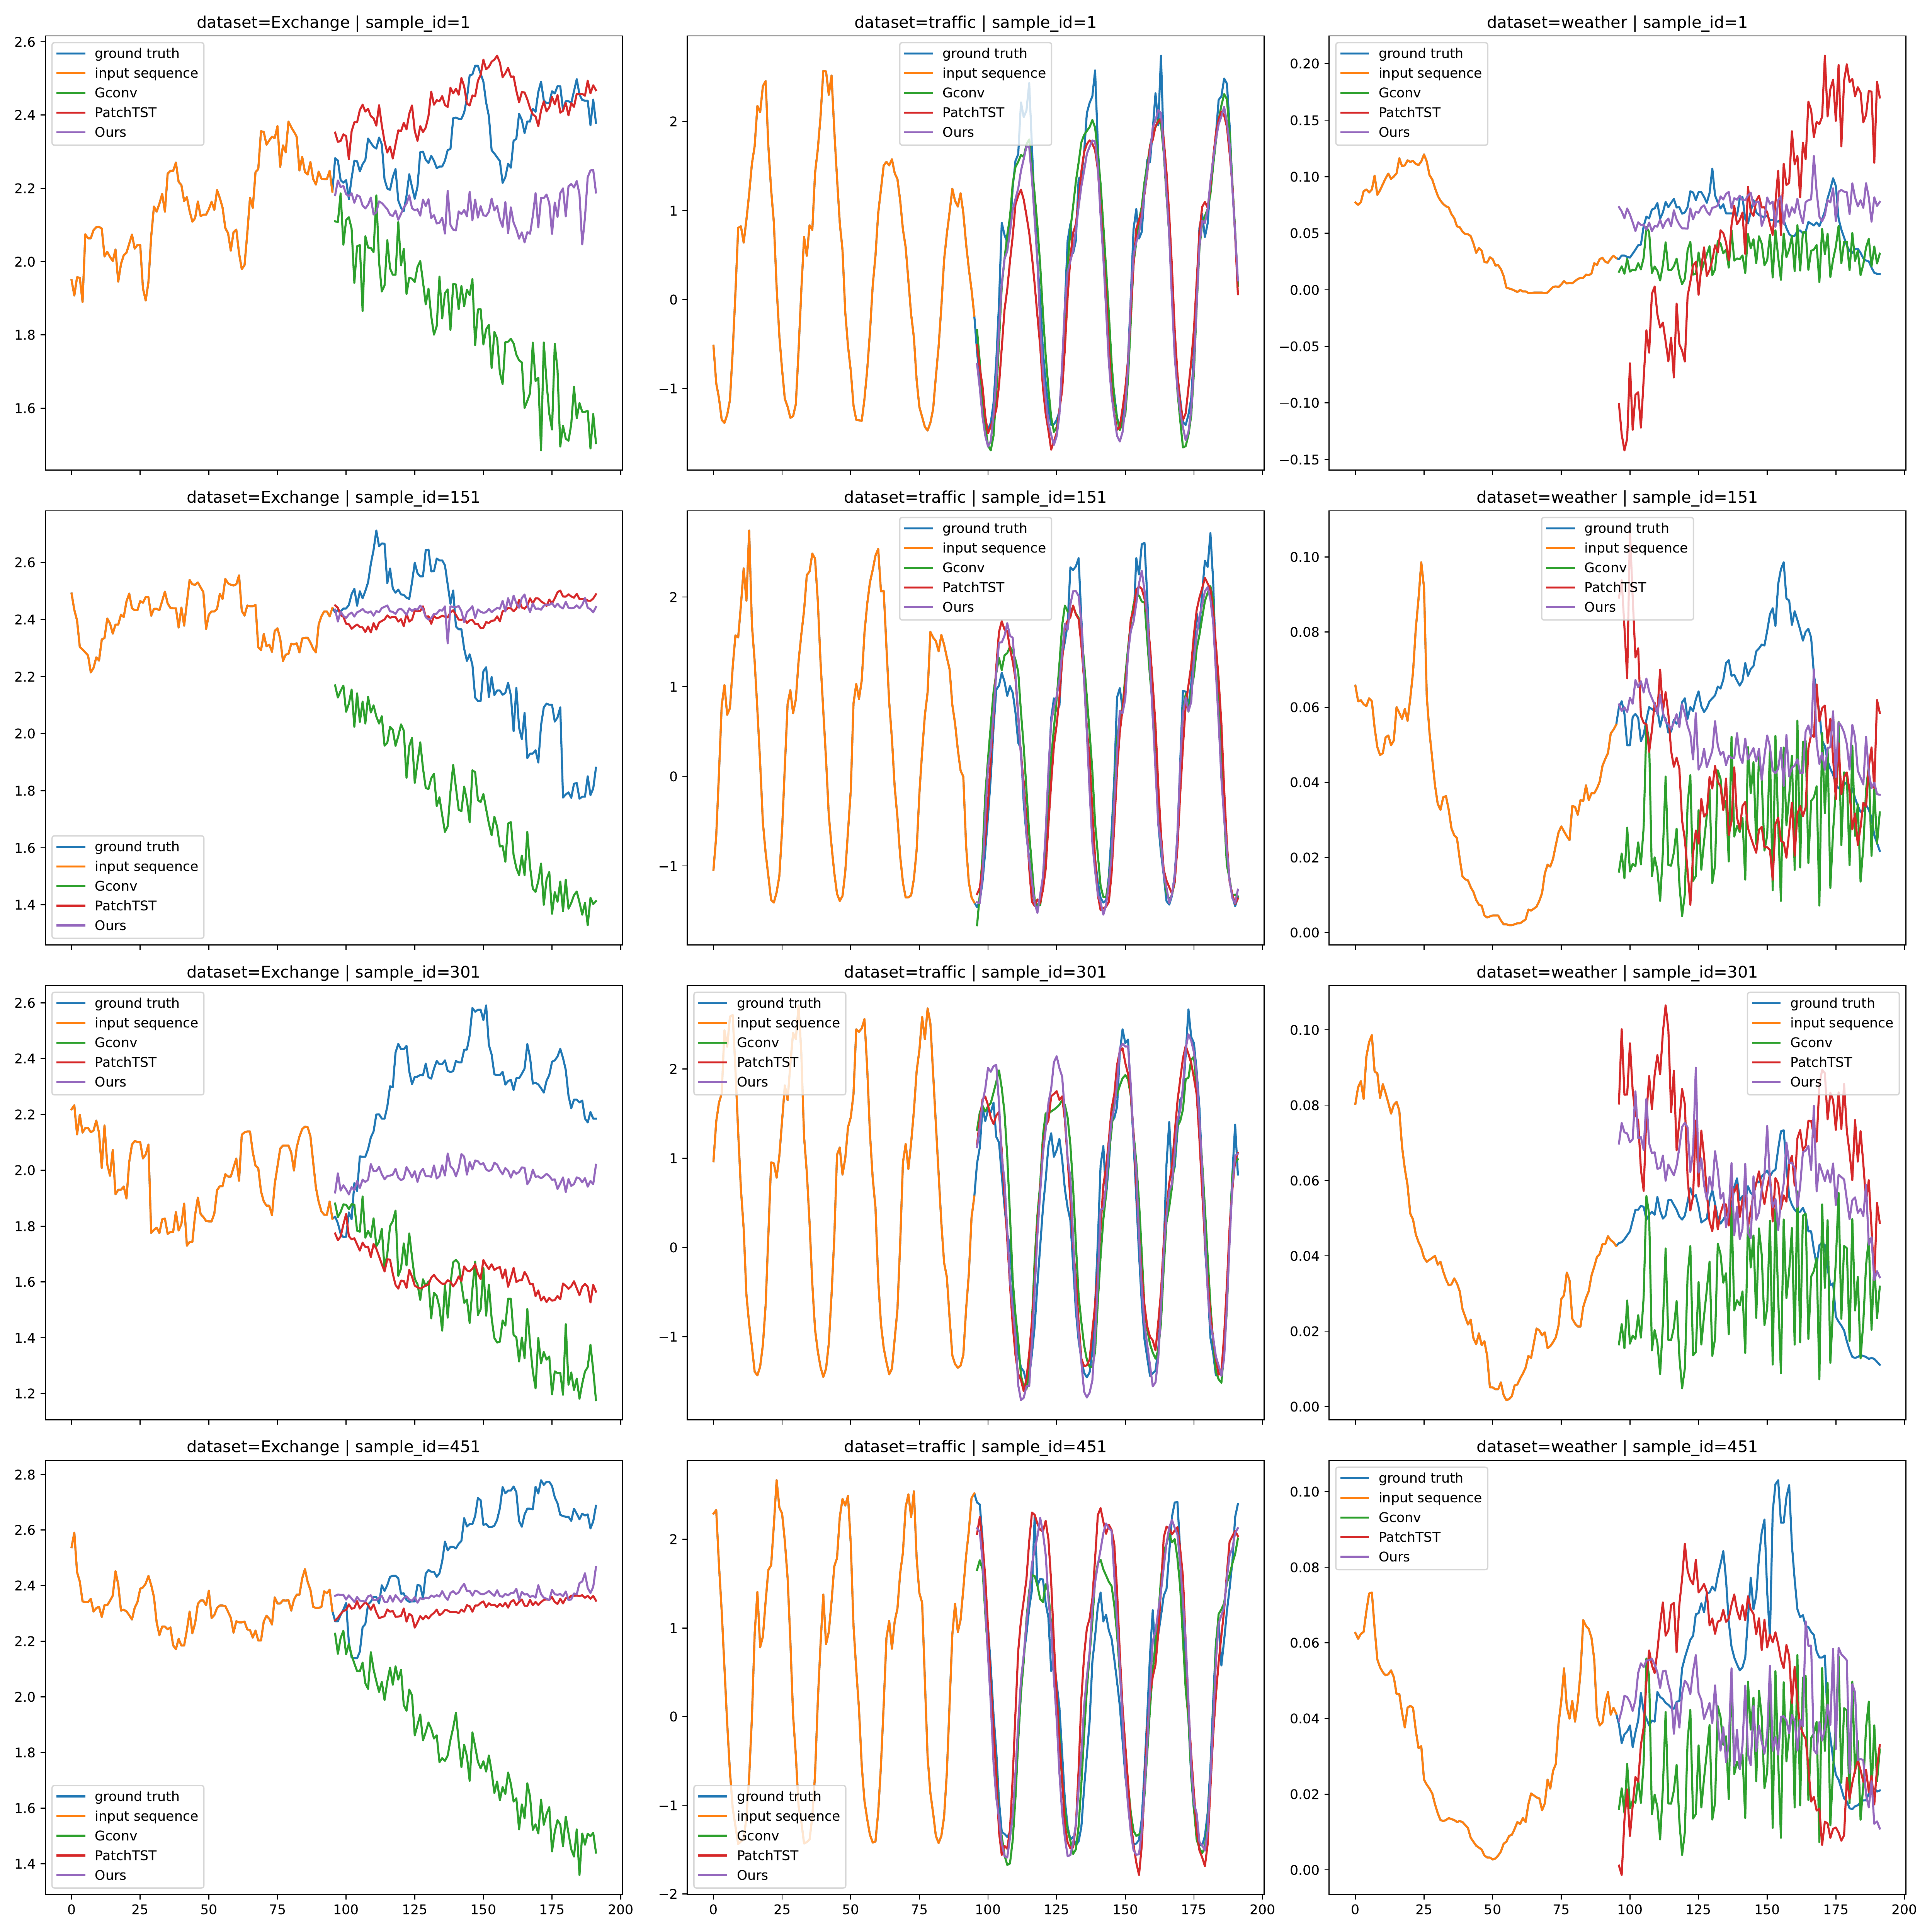}
\caption{.}
\label{fig:boost}
% \vskip -0.2in
\end{figure*}

We visualize the forecasting results of,

We observe that xxx.
