# Supplementary material for: GCformer: An Efficient Framework for Accurate and Scalable Long-Term Multivariate Time Series Forecasting
Source: arXiv:2306.08325 source file (2023-08-15)
Supplement: Supplementary file 6 [file algorithms.tex]

\section{Algorithm Implementation}
\label{app:Alg}
\input{figures/algorithm_0}
%\paragraph{Implementation for Frequency Enhanced Layer}
\input{figures/algorithm_1}
