# Supplementary material for: GCformer: An Efficient Framework for Accurate and Scalable Long-Term Multivariate Time Series Forecasting
Source: arXiv:2306.08325 source file (2023-08-15)
Supplement: Supplementary file 7 [file dataset_implmentation.tex]

\section{Dataset and Implementation Details}
\label{app:section_dataset_implem}
\subsection{Dataset Details}
\label{app:dataset}
In this subsection, we summarize the details of the datasets used in this paper as follows: 1) ETT~\cite{haoyietal-informer-2021} dataset contains two sub-dataset: ETT1 and ETT2, collected from two separated counties. Each of them has two versions of sampling resolutions (15min \& 1h). ETT dataset contains multiple time series of electrical loads and one time sequence of oil temperature. 2) Electricity\footnote{https://archive.ics.uci.edu/ml/datasets/ElectricityLoadDiagrams 20112014} dataset contains the electricity consumption for more than three hundred clients with each column corresponding to one client. 3) Exchange~\cite{lai2018modeling-exchange-dataset} dataset contains the current exchange of eight countries. 4) Traffic\footnote{http://pems.dot.ca.gov} dataset contains the occupation rate of freeway systems in California, USA. 5) Weather\footnote{https://www.bgc-jena.mpg.de/wetter/} dataset contains 21 meteorological indicators for a range of one year in Germany. 6) Illness\footnote{https://gis.cdc.gov/grasp/fluview/fluportaldashboard.html} dataset contains the influenza-like illness patients in the United States. Table \ref{tab:dataset} 
\input{tables/tab_dataset}
summarizes all the features of the six benchmark datasets. They are all split into the training set, validation set, and test set by the ratio of 7:1:2 during modeling.

\subsection{Implementation Details}
\label{app:exp:implement}
Our model is trained using ADAM \cite{kingma_adam:_2017} optimizer with a learning rate of $1e^{-4}$ to  $1e^{-3}$. The batch size is set to 32 (It depends on the GPU memory used in the experiment. In fact, a batch size up to 256 does not deteriorate the performance but with faster training speed if larger memory GPU or multiple GPUs is used). The default training process is 15 epochs without any early stopping. We save the model with the lowest loss on the validation set for the final testing. The mean square error (MSE) and mean absolute error (MAE) are used as metrics. All experiments are repeated 5 times and the mean of the metrics is reported as the final results. All the deep learning networks are implemented using PyTorch \cite{NEURIPS2019_9015_pytorch} and trained on NVIDIA V100 32GB GPUs/NVIDIA V100 16GB GPUs.

\subsection{Experiment Error Bars}
We train our model 5 times and calculate the error bars for FiLM and SOTA model FEDformer to compare the robustness, which is summarized in Table~\ref{tab:std}. It can be seen that the overall performance of the proposed FiLM is better than that of the SOTA FEDformer model.

\label{app:error_bars}
\vspace{-.2cm}
\begin{table}[ht]
%\setlength{\uppercaptionskip}{0.pt}
%\setlength{\belowcaptionskip}{-0.pt}
% \label{sample-table-kstest}
%\vskip 0.15in
\centering
\caption{MSE with error bars (Mean and STD) for FiLM and FEDformer baseline for multivariate long-term forecasting. All experiments are repeated 5 times.}
\begin{small}
% \begin{sc}
\scalebox{0.75}{
\begin{tabular}{c|c|ccccc}
\toprule
\multicolumn{2}{c|}{MSE}& ETTm2 & Electricity & Exchange & Traffic\\ %&\multicolumn{2}{c|}{Fedformer-f }\\%&\multicolumn{2}{c|}{}&\\
\midrule
\multirow{4}{*}{\rotatebox{90}{FiLM}} 
& 96 & 0.165 $\pm$ 0.0051 & 0.153$\pm$ 0.0014 & 0.079$\pm$ 0.002 & 0.416$\pm$ 0.010 \\
& 192 & 0.222 $\pm$ 0.0038 & 0.165$\pm$ 0.0023 & 0.159$\pm$ 0.011 & 0.408$\pm$ 0.007 \\
& 336 & 0.277 $\pm$ 0.0021 & 0.186$\pm$ 0.0018 & 0.270$\pm$ 0.018 & 0.425$\pm$ 0.007 \\
& 720 & 0.371 $\pm$ 0.0066 & 0.236$\pm$ 0.0022 & 0.536$\pm$ 0.026 & 0.520$\pm$ 0.003 \\
\midrule
\multirow{4}{*}{\rotatebox{90}{FED-f}} 
& 96 & 0.203 $\pm$ 0.0042 & 0.194 $\pm$ 0.0008 & 0.148 $\pm$ 0.002 & 0.217 $\pm$ 0.008 \\
& 192 & 0.269 $\pm$ 0.0023 & 0.201$\pm$ 0.0015 & 0.270$\pm$ 0.008 & 0.604 $\pm$ 0.004 \\
& 336 & 0.325 $\pm$ 0.0015 & 0.215$\pm$ 0.0018 & 0.460$\pm$ 0.016 & 0.621 $\pm$ 0.006 \\
& 720 & 0.421 $\pm$ 0.0038 & 0.246$\pm$ 0.0020 & 1.195$\pm$ 0.026 & 0.626 $\pm$ 0.003 \\
\bottomrule
\end{tabular}
}
\label{tab:std}
% \end{sc}
\end{small}
%\end{center}
\vskip -0.1in
\end{table}

\subsection{Univariate Forecasting Results}
\label{app:exp:uni_bench}
The univariate benchmark results are summarized in Table~\ref{tab:uni-benchmarks-large}.
\begin{table*}[h]
% \begin{adjustwidth}{-1.5in}{-1in}
\centering
%\begin{small}
\caption{Univariate long-term forecasting results on six datasets with various input length and prediction horizon $O \in \{96,192,336,720\}$. A lower MSE indicates better performance. All experiments are repeated 5 times.}
\vskip 0.05in
\scalebox{0.60}{
\begin{tabular}{c|c|cccccccccccccc}
\toprule
\multicolumn{2}{c|}{Methods}&\multicolumn{2}{c|}{FiLM}&\multicolumn{2}{c|}{FEDformer}&\multicolumn{2}{c|}{Autoformer}&\multicolumn{2}{c|}{S4}&\multicolumn{2}{c|}{Informer}&\multicolumn{2}{c|}{LogTrans}&\multicolumn{2}{c}{Reformer}\\
\midrule
\multicolumn{2}{c|}{Metric} & MSE  & MAE & MSE & MAE& MSE  & MAE& MSE  & MAE& MSE  & MAE& MSE  & MAE& MSE  & MAE\\
\midrule
\multirow{4}{*}{\rotatebox{90}{$ETTm2$}} 
& 96 & 0.065 &\textbf{0.189}  &\textbf{0.063} &0.189 & 0.065 & 0.189 &0.153 &0.318 & 0.088 & 0.225 & 0.075 & 0.208 & 0.076  &0.214   \\
& 192 & \textbf{0.094} & \textbf{0.233} &0.102 &0.245 & 0.118 & 0.256 &0.183 &0.350 & 0.132 &0.283 & 0.129 &0.275  & 0.132  & 0.290   \\
& 336 & \textbf{0.124} & \textbf{0.274} &0.130 &0.279 & 0.154 & 0.305 &0.204 & 0.367 &0.180 &0.336 & 0.154 &0.302  & 0.160  & 0.312    \\
& 720 & \textbf{0.173} & \textbf{0.323} &0.178 &0.325 & 0.182 &0.335 &0.482 &0.567  &0.300  &0.435 & 0.160 &0.321  & 0.168  &0.335     \\
\midrule
\multirow{4}{*}{\rotatebox{90}{$Electricity$}} 
& 96  & \textbf{0.154} & \textbf{0.247} &0.253 &0.370  &0.341 &0.438 &0.351 &0.452 & 0.484& 0.538 &0.288& 0.393& 0.274 & 0.379   \\
& 192 & \textbf{0.166} & \textbf{0.258} &0.282 &0.386 &0.345 &0.428 &0.373 &0.455 & 0.557& 0.558 &0.432 & 0.483 & 0.304 &0.402   \\
& 336 & \textbf{0.188} & \textbf{0.283} &0.346 &0.431 &0.406 &0.470 &0.408 &0.477 & 0.636& 0.613 &0.430 &0.483 & 0.370 &0.448  \\
& 720 & \textbf{0.249} & \textbf{0.341} &0.422 &0.484 &0.565 &0.581 &0.472 &0.517 & 0.819& 0.682 &0.491 &0.531 & 0.460 &0.511   \\
\midrule

\multirow{4}{*}{\rotatebox{90}{$Exchange$}} 
&96  & \textbf{0.110} & \textbf{0.259} &0.131 &0.284 & 0.241 & 0.387 &0.344 &0.482  & 0.591  &0.615  &0.237 &0.377  &0.298  &0.444    \\
& 192 & \textbf{0.207} & \textbf{0.352} &0.277 &0.420 &0.300  &0.369 &0.362 &0.494  &1.183   &0.912 &0.738  &0.619  &0.777  & 0.719   \\
& 336 & \textbf{0.327} & \textbf{0.461} &0.426 &0.511 &0.509  &0.524 &0.499 &0.594  &1.367  &0.984  &2.018  &1.070  &1.832  &1.128     \\
& 720 & \textbf{0.811} & \textbf{0.708} &1.162 &0.832 &1.260  &0.867 &0.552 & 0.614 &1.872  &1.072  &2.405  &1.175  &1.203  &0.956     \\
\midrule
\multirow{4}{*}{\rotatebox{90}{$Traffic$}} 
&96  & \textbf{0.144} & \textbf{0.215} &0.170 &0.263  &0.246 &0.346 &0.194 &0.290 & 0.257 & 0.353 &0.226 &0.317 &  0.313 & 0.383\\
& 192 & \textbf{0.120} & \textbf{0.199} &0.173 &0.265 &0.266 &0.370 &0.172 &0.272 & 0.299 & 0.376 &0.314 &0.408 & 0.386 & 0.453\\
& 336 & \textbf{0.128} & \textbf{0.212} &0.178 &0.266 &0.263 &0.371 &0.178 &0.278 & 0.312 & 0.387 &0.387 &0.453 & 0.423 & 0.468\\
& 720 & \textbf{0.153} & \textbf{0.252} &0.187 &0.286 &0.269 &0.372 &0.263 &0.386 & 0.366 & 0.436 &0.491 &0.437 & 0.378 & 0.433\\
\midrule
\multirow{4}{*}{\rotatebox{90}{$Weather$}}
& 96  & \textbf{0.0012} & \textbf{0.026} & 0.0035 & 0.046 & 0.011 &0.081 &0.0061 &0.065 & 0.0038 & 0.044 & 0.0046 &0.052 & 0.012 & 0.087 \\
& 192 & \textbf{0.0014}& \textbf{0.029}&0.0054 &0.059 &0.0075 &0.067 &0.0067 &0.067 & 0.0023 & 0.040 &0.0056 & 0.060 & 0.0098 & 0.079  \\
& 336 & \textbf{0.0015} & \textbf{0.030} &0.0041 &0.050 &0.0063 &0.062 &0.0025 &0.0381 & 0.0041 & 0.049 &0.0060 &0.054& 0.0050 & 0.059 \\
& 720 & \textbf{0.0022} & \textbf{0.037} &0.015 &0.091 &0.0085 &0.070 &0.0074 &0.0736 & 0.0031 & 0.042 &0.0071 &0.063& 0.0041 & 0.049 \\
\midrule
\multirow{4}{*}{\rotatebox{90}{$ILI$}} 
& 24 & \textbf{0.629} & \textbf{0.538} &0.693 &0.629 &0.948 &0.732 &0.866 &0.584 & 5.282 &2.050 &3.607 & 1.662 & 3.838 & 1.720  \\
& 36 & \textbf{0.444} & \textbf{0.481} &0.554 &0.604 &0.634 &0.650 &0.622 &0.532 & 4.554 &1.916 &2.407 & 1.363 & 2.934 & 1.520 \\
& 48 & \textbf{0.557} & \textbf{0.584} &0.699 &0.696 &0.791 &0.752 &0.813 &0.679 & 4.273 &1.846 &3.106 & 1.575 & 3.754 & 1.749\\
& 60 & \textbf{0.641} & \textbf{0.644} &0.828 &0.770 &0.874 &0.797 &0.931 &0.747 & 5.214 &2.057 &3.698 & 1.733 & 4.162 & 1.847\\
\bottomrule
\end{tabular}
}
\label{tab:uni-benchmarks-large}
\vskip -0.10in
% \end{adjustwidth}
%\end{small}tab:multi-benchmarks
\end{table*}

\subsection{ETT Full Benchmark}
\label{app:exp:ett_benchmark}
We present the full-benchmark on four ETT datasets \cite{haoyietal-informer-2021} in Table \ref{tab:multi-benchmarks-ett} (multivariate forecasting) and Table \ref{tab:uni-benchmarks-ett} (univariate forecasting). The ETTh1 and ETTh2 are recorded hourly while ETTm1 and ETTm2 are recorded every 15 minutes. The time series in ETTh1 and ETTm1 follow the same pattern, and the only difference is the sampling rate, similarly for ETTh2 and ETTm2. On average, our 
FiLM yields a \textbf{14.0\%} relative MSE reduction for multivariate forecasting, and a \textbf{16.8\%} reduction for univariate forecasting over the SOTA results from FEDformer.
\label{app:ETT}

\begin{table*}[h]
\centering
% \begin{small}
% \begin{adjustwidth}{-1.5in}{-1in}
\caption{Multivariate long-term forecasting results on ETT full benchmark. The best results are highlighted in bold. A lower MSE indicates better performance. All experiments are repeated 5 times.}
\vskip 0.05in
\scalebox{0.75}{
\begin{tabular}{c|c|cccccccccccccccccc}
\toprule
\multicolumn{2}{c|}{Methods}&\multicolumn{2}{c|}{FiLM}&\multicolumn{2}{c|}{FEDformer}&\multicolumn{2}{c|}{Autoformer}&\multicolumn{2}{c|}{S4}&\multicolumn{2}{c|}{Informer}&\multicolumn{2}{c|}{LogTrans}&\multicolumn{2}{c}{Reformer}\\
\midrule
\multicolumn{2}{c|}{Metric} & MSE  & MAE & MSE & MAE& MSE  & MAE& MSE  & MAE& MSE  & MAE& MSE  & MAE& MSE  & MAE\\
\midrule
\multirow{4}{*}{\rotatebox{90}{$ETTh1$}}
& 96 &\textbf{0.371} &\textbf{0.394} &0.376 &0.419  & 0.449& 0.459 &0.949 &0.777 & 0.865 & 0.713& 0.878& 0.740& 0.837& 0.728\\
& 192 &\textbf{0.414} &\textbf{0.423} &0.420 &0.448  & 0.500& 0.482 &0.882 &0.745 & 1.008 & 0.792& 1.037& 0.824& 0.923& 0.766\\
& 336 &\textbf{0.442} &\textbf{0.445} &0.459 &0.465  & 0.521& 0.496 &0.965 &0.75 & 1.107 & 0.809& 1.238& 0.932& 1.097& 0.835\\
& 720 &\textbf{0.465} &\textbf{0.472} &0.506 &0.507  & 0.514& 0.512 &1.074&0.814 & 1.181 &0.865&  1.135& 0.852& 1.257& 0.889\\
\midrule
\multirow{4}{*}{\rotatebox{90}{$ETTh2$}}
& 96  &\textbf{0.284} &\textbf{0.348} &0.346 &0.388 & 0.358& 0.397 &1.551&	0.968 & 3.755& 1.525& 2.116& 1.197 &2.626 &1.317\\
& 192 &\textbf{0.357} &\textbf{0.400} &0.429 &0.439 & 0.456& 0.452 &2.336	 &1.229 & 5.602& 1.931& 4.315& 1.635 &11.12 &2.979\\
& 336 &\textbf{0.377} &\textbf{0.417} &0.482 &0.480 & 0.482& 0.486 &2.801	 &1.259 & 4.721& 1.835& 1.124& 1.604 &9.323 &2.769\\
& 720 &\textbf{0.439} &\textbf{0.456} & 0.463 & 0.474 & 0.515& 0.511 &2.973	 &1.333 & 3.647& 1.625& 3.188& 1.540 &3.874 &1.697\\
\midrule
\multirow{4}{*}{\rotatebox{90}{$ETTm1$}}
& 96  &\textbf{0.302} &\textbf{0.345} &0.378 &0.418 & 0.505& 0.475 &0.640	 &0.584 & 0.672& 0.571& 0.600& 0.546 &0.538 &0.528\\
& 192 &\textbf{0.338} &\textbf{0.368} & 0.426 & 0.441 & 0.553& 0.496 &0.570	 &0.555 & 0.795& 0.669& 0.837& 0.700 &0.658 &0.592\\
& 336 &\textbf{0.373} &\textbf{0.388} & 0.445 & 0.459 & 0.621& 0.537 &0.795& 0.691& 1.212& 0.871& 1.124& 0.832 &0.898 &0.721\\
& 720 &\textbf{0.420} &\textbf{0.420} & 0.543 & 0.490 & 0.671& 0.561 &0.738 &0.655 & 1.166& 0.823& 1.153& 0.820 &1.102 &0.841\\
\midrule
\multirow{4}{*}{\rotatebox{90}{$ETTm2$}} &96 &\textbf{0.165} &\textbf{0.256} & 0.203 & 0.287 &0.255  &0.339  &0.705	 &0.690  &0.365  &0.453  &0.768  &0.642  &0.658  &0.619 \\
                        & 192 &\textbf{0.222} &\textbf{0.296} & 0.269 & 0.328 &0.281 &0.340  &0.924	 &0.692 &0.533  &0.563  &0.989  &0.757  &1.078  &0.827 \\
                        & 336 &\textbf{0.277} &\textbf{0.333} & 0.325 & 0.366  &0.339  &0.372  &1.364	 & 0.877 &1.363&0.887  &1.334  &0.872  &1.549  &0.972 \\
                        & 720 &\textbf{0.371} &\textbf{0.389} & 0.421 & 0.415  &0.422  &0.419  &2.074 &1.074  &3.379  &1.338 & 3.048 &1.328  &2.631  &1.242 \\
\bottomrule
\end{tabular}
}
\label{tab:multi-benchmarks-ett}
% \end{adjustwidth}
% \end{small}
% \vskip -0.1in
\end{table*}

\begin{table*}[h]
\centering
% \begin{small}
% \begin{adjustwidth}{-1.5in}{-1in}
\caption{Univariate long-term forecasting results on ETT full benchmark. The best results are highlighted in bold. A lower MSE indicates better performance. All experiments are repeated 5 times.}
\vskip 0.05in
\scalebox{0.75}{
\begin{tabular}{c|c|cccccccccccccccccc}
\toprule
\multicolumn{2}{c|}{Methods}&\multicolumn{2}{c|}{FiLM}&\multicolumn{2}{c|}{FEDformer}&\multicolumn{2}{c|}{Autoformer}&\multicolumn{2}{c|}{S4}&\multicolumn{2}{c|}{Informer}&\multicolumn{2}{c|}{LogTrans}&\multicolumn{2}{c}{Reformer}\\
\midrule
\multicolumn{2}{c|}{Metric} & MSE  & MAE & MSE & MAE& MSE  & MAE& MSE  & MAE& MSE  & MAE& MSE  & MAE& MSE  & MAE\\
\midrule

\multirow{4}{*}{\rotatebox{90}{$ETTh1$}}
&96 &\textbf{0.055}&\textbf{0.178}&0.079 &0.215 &0.071 &0.206 &0.316 &0.490 &	0.193&	0.377&	0.283&	0.468&	0.532&	0.569\\
&192 &\textbf{0.072}&\textbf{0.207}&0.104 &0.245 & 0.114&	0.262 & 0.345&0.516 &	0.217&	0.395&	0.234&	0.409&	0.568&	0.575\\
&336 &\textbf{0.083}&\textbf{0.229}&0.119 &0.270 &0.107&0.258 &0.825 &0.846 &	0.202&	0.381&	0.386&	0.546&	0.635&	0.589\\
&720 &\textbf{0.090}&\textbf{0.240}&0.127 &0.280 &0.126&0.283 &0.190 &0.355 &	0.183&	0.355&	0.475&	0.628&	0.762&	0.666\\
\midrule
\multirow{4}{*}{\rotatebox{90}{$ETTh2$}}
&96 &\textbf{0.127}&0.272&0.128 &\textbf{0.271} & 0.153&	0.306 & 0.381&0.501 &	0.213&	0.373&	0.217&	0.379&	1.411&	0.838\\
&192 &\textbf{0.182}&0.335&0.185 &\textbf{0.330} & 0.204&	0.351 & 0.332&0.458 &	0.227&	0.387&	0.281&	0.429&	5.658&	1.671\\
&336 &\textbf{0.204}&\textbf{0.367}&0.231 &0.378 & 0.246&	0.389 & 0.655&0.670 &	0.242&	0.401&	0.293&	0.437&	4.777&	1.582\\
&720 &\textbf{0.241}&\textbf{0.396}&0.278 &0.420 & 0.268&	0.409 & 0.630&0.662 &	0.291&	0.439&	0.218&	0.387&	2.042&	1.039\\
\midrule
\multirow{4}{*}{\rotatebox{90}{$ETTm1$}}
&96 &\textbf{0.029}&\textbf{0.127}&0.033 &0.140 & 0.056&	0.183 & 0.651&0.733 &	0.109&	0.277&	0.049&	0.171&	0.296&	0.355\\
&192 &\textbf{0.041}&\textbf{0.153}&0.058 &0.186 & 0.081&	0.216 & 0.190& 0.372&	0.151&	0.310&	0.157&	0.317&	0.429&	0.474\\
&336 &\textbf{0.053}&\textbf{0.175}&0.071 &0.209 & 0.076&	0.218 & 0.428&0.581 &	0.427&	0.591&	0.289&	0.459&	0.585&	0.583\\
&720 &\textbf{0.071}&\textbf{0.205}&0.102 &0.250 & 0.110&	0.267 & 0.254&0.433 &	0.438&	0.586&	0.430&	0.579&	0.782&	0.730\\
\midrule
\multirow{4}{*}{\rotatebox{90}{$ETTm2$}} 
& 96 &0.065&\textbf{0.189}&\textbf{0.063} &0.189 & 0.065 & 0.189  & 0.153&0.318 & 0.088 & 0.225 & 0.075 & 0.208 & 0.076  &0.214   \\
& 192 &\textbf{0.094}&\textbf{0.233}& 0.102 & 0.245 & 0.118 & 0.256  &0.183 &0.350 & 0.132 &0.283 & 0.129 &0.275  & 0.132  & 0.290   \\
& 336 &\textbf{0.124}&\textbf{0.274}& 0.130 & 0.279 & 0.154 & 0.305  &0.204 &0.367  &0.180 &0.336 & 0.154 &0.302  & 0.160  & 0.312    \\
& 720 &\textbf{0.173}&\textbf{0.323}& 0.178 & 0.325 & 0.182 &0.335  &0.482 &0.567  &0.300  &0.435 & 0.160 &0.321  & 0.168  &0.335     \\
\bottomrule
\end{tabular}
}
\label{tab:uni-benchmarks-ett}
% \end{adjustwidth}
% \end{small}
\end{table*}
