# Supplementary material for: GCformer: An Efficient Framework for Accurate and Scalable Long-Term Multivariate Time Series Forecasting
Source: arXiv:2306.08325 source file (2023-08-15)
Supplement: Supplementary file 8 [file distribution.tex]

\section{Distribution Analysis of Forecasting Output}
\label{app:Distribution}
\subsection{Kolmogorov-Smirnov Test}
We adopt the Kolmogorov-Smirnov (KS) test to check whether our model's input and output sequences come from the same distribution. The KS test is a nonparametric test for checking the equality of probability distributions. In essence, the test answers the following question ``Are these two sets of samples drawn from the same distribution?''. 
The Kolmogorov-Smirnov statistic is defined as:
$$
D_{n, m}=\sup _{x}\left|F_{1, n}(x)-F_{2, m}(x)\right|, 
$$
where $\sup$ is the supremum function, $F_{1, n}$ and $F_{2, m}$ are the empirical distribution functions of the two compared samples.
For samples that are large enough, the null hypothesis would be rejected at level $\alpha$ if
$$
D_{n, m}>\sqrt{-\frac{1}{2}\ln \left(\frac{\alpha}{2}\right)} \cdot \sqrt{\frac{n+m}{n \cdot m}},
$$
where $n$ and $m$ are the first and second sample sizes.
\subsection{Distribution Analysis}
In this section, we evaluate the distribution similarity between models' input and output sequences using the KS test. In Table \ref{tab:KStest_small}, we applied the Kolmogrov-Smirnov test to check if the output sequences of various models that trained on ETTm1/ETTm2 are consistent with the input sequence. 
%This method is better used on some stationary time series datasets such as electric load forecast. 
On both datasets, by setting the standard P-value as 0.01, various existing baseline models have much smaller P-values except FEDformer and Autoformer, which indicates their outputs have a high probability of being sampled from different distributions compared to their input signals. Autoformer and FEDformer have much larger P-values mainly due to their seasonal-trend decomposition mechanism. The proposed FiLM also has a much larger P-value compared to most baseline models. And its null hypothesis can not be rejected in most cases for these two datasets. It implies that the output sequence generated by FiLM shares a similar pattern as the input signal, and thus justifies our design motivation of FiLM as discussed in Section~\ref{sec_intro}. Though FiLM gets a smaller P-value than FEDformer, it is close to the actual output, which indicates that FiLM makes a good balance between recovering and forecasting. 

\begin{table}[h]
%\setlength{\uppercaptionskip}{0.pt}
%\setlength{\belowcaptionskip}{-0.pt}
%\vskip 0.15in
\centering
\caption{P-values of Kolmogrov-Smirnov test of different Transformer models for long-term forecasting output on ETTm1 and ETTm2 dataset. Larger value indicates the hypothesis (the input sequence and forecasting output come from the same distribution) is less likely to be rejected. The largest results are highlighted.}
\begin{small}
% \begin{sc}
\vskip 0.05in
\scalebox{0.80}{
\begin{tabular}{c|c|cccccc}
\toprule
\multicolumn{2}{c|}{Methods}&Transformer&Informer&Autoformer&FEDformer&FiLM&True\\ %&\multicolumn{2}{c|}{Fedformer-f }\\%&\multicolumn{2}{c|}{}&\\
\midrule
\multirow{4}{*}{\rotatebox{90}{ETTm1}} 
& 96 & 0.0090 & 0.0055&0.020 & \textbf{0.048} & 0.016& {0.023} \\
& 192 & 0.0052 & 0.0029&0.015 & \textbf{0.028} & 0.0123& {0.013} \\
& 336 & 0.0022 & 0.0019&0.012 & \textbf{0.015} & 0.0046& {0.010} \\
% & 720 & 0.0023 & 0.0016 & \textbf{0.014} & \textbf{0.0036} \\
& 720 & 0.0023 & 0.0016&0.008 & \textbf{0.014} & 0.0024& {0.004} \\
\midrule
\multirow{4}{*}{\rotatebox{90}{ETTm2}} 
% & 48 & 0.454 & & 0.366 & & 0.476 & & 0.356 \\
& 96 & 0.0012 & 0.0008& \textbf{0.079} &{0.071} & 0.022 & {0.087} \\%& \textbf{0.379} & \textbf{0.419}\\
& 192 & 0.0011 & 0.0006& \textbf{0.047} &{0.045}  &0.020 & {0.060} \\%& \textbf{0.426} & \textbf{0.441}\\
% & 288 & 0.634 & & 0.430 & & 0.571 & & 0.379 \\
& 336 & 0.0005 & 0.00009& 0.027 &\textbf{0.028} &0.012 & {0.042} \\%& \textbf{0.445} & \textbf{0.459}\\
% & 672 & 0.606 & & 0.528 & & 0.544 & & 0.501\\
& 720 & 0.0008& 0.0002& \textbf{0.023} & {0.021} &0.0081 & {0.023} \\
% \multicolumn{2}{c|}{Count}& 0 & 0 & 3 & 5 & 7& NA \\
%& \textbf{0.543} & \textbf{0.490}\\
%& -96 & 0.0012 & 0.0009 & 0.0001 & 0.0037 & \textbf{0.039} & \textbf{0.012} \\
\bottomrule
\end{tabular}
}
\label{tab:KStest_small}
% \end{sc}
\end{small}
%\end{center}
\vskip -0.1in
\end{table}
