# Supplementary material for: GCformer: An Efficient Framework for Accurate and Scalable Long-Term Multivariate Time Series Forecasting
Source: arXiv:2306.08325 source file (2023-08-15)
Supplement: Supplementary file 9 [file mode_selection.tex]

% \section{Mode Selection Policy for FEL}
% \label{app:mode}
% Three different mode selection policies are studied for frequency enhanced layer: 1) lowest mode selection: we select $m$ lowest frequency modes to retain. 2) random model selection: we select $m$ frequency modes randomly to retain. 3) lowest with extra high mode selection: we select $0.8\times m$ lowest frequency modes and $0.2\times m$ high frequency modes randomly to retain. The experimental results are summarized in Table \ref{tab:mode} with $m = 32$ for both experiments.
% \input{tables/tab_mode_selection_policy}
