# Supplementary material for: GCformer: An Efficient Framework for Accurate and Scalable Long-Term Multivariate Time Series Forecasting
Source: arXiv:2306.08325 source file (2023-08-15)
Supplement: Supplementary file 13 [file related_work.tex]

\section{Related Work}
\label{App:related_works}
In this section, we will give an overview of the related literature in time series forecasting. %The relevant work includes traditional times series models (\ref{App:related_work_tradi_time}), deep learning models (\ref{App:related_work_tradi_time}), Transformer-based models (\ref{App:related_work_transformers}), and the Fourier Transform in neural networks (\ref{App:related_work_fft}).

% \subsection{General Time-line of Time Series Models}
% \label{App:related_work_tradi_time}

%Data-driven time series forecasting helps researchers understand the evolution of the systems without architecting the exact physics law behind them. After decades of renovation, time series models have been well developed and served as the backbone of various projects in numerous application fields. 

\paragraph{Traditional Time Series Models} The first generation of well-discussed time series model is the autoregressive family. ARIMA~\cite{box_arima2,box_distribution_1970} follows the Markov process and build recursive sequential forecasting. However, a plain autoregressive process has difficulty in dealing non-stationary sequences. Thus, ARIMA employed a pre-process iteration by differencing, which transforms the series to stationary. Still, ARIMA and related models have the linear assumption in the autoregressive process, which limits their usage in complex forecasting tasks. 

\paragraph{Deep Neural Network in Forecasting}
With the bloom of deep neural networks, recurrent neural networks (RNNs) were designed for tasks involving sequential data. However, canonical RNN tends to suffer from gradient vanishing/exploding problems with long input because of its recurrent structure. Among the family of RNNs, LSTM~\cite{hochreiter_long_1997_lstm} and GRU~\cite{GRU_cho_et_al_2014} proposed gated structure to control the information flow to deal with the gradient vanishing/exploration problem. Although recurrent networks enjoy fast inference, they are slow to train and not parallelizable. Temporal convolutional network (TCN)~\cite{Think_globally_act_locally_tcn_time_series_2019} is another family for sequential tasks. However, limited to the reception field of the kernel, the long-term dependencies are hard to capture. Convolution is a parallelizable operation but expensive in inference.

\paragraph{Transformers}
With the innovation of Transformers in natural language processing~\cite{attention_is_all_you_need,Bert/NAACL/Jacob} and in computer vision tasks~\cite{Transformers-for-image-at-scale/iclr/DosovitskiyB0WZ21,DBLP:Global-filter-FNO-in-cv}, they are also discussed, renovated, and applied in time series forecasting~\cite{wen2022transformers}, especially the main attention module. Some works use temporal attention~\cite{dual-state-attention-rnn-qin} to capture long-range dependencies for time series. Others use the backbone of Transformer. Transformers usually employ an encoder-decoder architecture, with the self-attention and cross-attention mechanisms serving as the core layers. \cite{Log-transformer-shiyang-2019} invents a logsparse attention module to deal with the memory bottleneck for Transformer model. \cite{DBLP:conf/iclr/KitaevKL20-reformer} uses locality-sensitive
hashing to replace the attention module for less time complexity. \cite{haoyietal-informer-2021} proposes a probability sparse attention mechanism to deal with long-term forecasting. \cite{Autoformer} designs a decomposition Transformer architecture with an Auto-Correlation mechanism as an alternative for the attention module. \cite{liu2022pyraformer} designs a low-complexity Pyramidal Attention for the long-term time forecasting tasks. \cite{FedFormer} proposes two attention modules that operate in the frequency domain using Fourier or wavelet transformation.

\paragraph{Orthogonal Basis and Neural Network}
Orthogonal basis project arbitrary functions onto a certain space and thus enable the representation learning in another view. Orthogonal basis family is easy to be discretized and serves as a plug-in operation in neural networks. Recent studies began to realize the efficiency and effectiveness of the Orthogonal basis, including the polynomial family and others (Fourier basis \& Multiwavelet basis). Fourier basis is first introduced for acceleration due to the Fast Fourier algorithm, for example, acceleration of computing convolution~\cite{Hippo} or Auto-correlation function~\cite{wen2021robustperiod,Autoformer}. Fourier basis also serves as a performance boosting block: Fourier with Recurrent structure~\cite{FourierRecurrentUnits}, Fourier with MLP~\cite{Fourier-Neural-Operator,FNet} and Fourier in Transformer~\cite{FedFormer}. Multiwavelet transform is a more local filter (compared with 
Fourier) and a frequency decomposer. Thus, neural networks which employ multiwavelet filter usually exhibit a hierarchical structure and treat different frequency in different tunnels, e.g., \cite{wang2018multilevel,Multiwavelet-based-Operator-Learning,FedFormer}. Orthogonal Polynomials are naturally good selections of orthogonal basis. Legendre Memory Unit (LMU)~\cite{LMU} uses Legendre Polynomials for an orthogonal projection of input signals for memory strengthening with the backbone of LSTM. The projection process is mathematically derived from delayed linear transfer function. HiPPO~\cite{Hippo}, based on LMU, proposes a novel mechanism (Scaled Legendre), which involves the function's full history (LMU uses rolling windowed history). In the subsequent work of HiPPO, the authors propose S4 model~\cite{S4} and give the first practice on time series forecasting tasks. However, LMU and HiPPO share the same backbone (LSTM), which may limit their performance. %Furthermore, the setting of Scale Legendre in HiPPO (history without decay) may not stand in time series forecasting.

% Legendre

% Laguerre

% ~\cite{FNet}

% \subsection{State Space Model}
% RFF is compact in \cite{Sampled-softmax-with-random-Fourier-Features/nips/RawatCYSK19}

% Optimal Rates for Random Fourier Features
