# Supplementary material for: GCformer: An Efficient Framework for Accurate and Scalable Long-Term Multivariate Time Series Forecasting
Source: arXiv:2306.08325 source file (2023-08-15)
Supplement: Supplementary file 14 [file theoretical_analysis.tex]

% 请见 proof_fourier 这一章，这两章重复了。

% \section{Theoretical Analysis}

% \subsection{Theorem 1}
% The proof is a simple extension of the Proposition 6 in \cite{Hippo}. We omit it for brevity.


% \subsection{Theorem 2}
% % In order to generate a stable sequence $\{x_t\}$, we restrict the matrix $A$ to be unitary. The above Theorem indicates that the uncertain portion between $x_{t}$  and its estimation $A^{\theta}x_{t-\theta} + \sum_{i=1}^{\theta-1}A^{i}b$ at time $t-\theta$ is scaled with $\sqrt{\theta}$. The larger $\theta$ will lead to higher uncertainty and it in turn leads less correlation between $x_t$ and $x_{t-\theta}$. Therefore introducing more historical information may not necessary lead better performance.

% \begin{align}
%     x_{t} &= Ax_{t-1} +  b + \epsilon_{t-1}\notag\\
%     &= A(Ax_{t-2} +  b + \epsilon_{t-2})+  b + \epsilon_{t-1}\notag\\
%     &=A^2x_{t-2} + Ab + b + A\epsilon_{t-2} + \epsilon_{t-1}\notag\\
%     % &=A^3x_{t-3} +  A^2b  + Ab + b + A^2\epsilon_{t-3}+ A\epsilon_{t-2} + \epsilon_{t-1}\notag\\
%     &\cdots\notag\\
%     &=A^{\theta}x_{t-\theta} + \sum_{i=1}^{\theta-1}A^ib+ \underbrace{\sum_{i=1}^{\theta-1}A^i\epsilon_{t-i}}_{(*)}\notag
% \end{align}
% Following Hoeffding inequality, for $\mu>0$ we have
% \begin{align}
%     \mathbbm{P}\left(|(*)|\ge \mu\right)\le \exp\left(-\frac{2\mu^2}{\sum_{i=1}^{\theta -1}\|A^i\epsilon_{t-1}\|_{\psi_2}^2}\right),
% \end{align}
% where $\|\cdot\|_{\psi_2}$ is the Orlicz norm defined as
% \begin{align}
%     \|X\|_{\psi_2} :=\inf\left\{c\ge 0: \mathbbm{E}[\exp(X^2/c^2)]\le 2\right\}\notag.
% \end{align}
% Since we require $A$ being unitary, we will have $\|A\epsilon\|_2^2 = \|\epsilon\|_2^2$ and it implies $\|A^i\epsilon_{t-1}\|_{\psi_2}^2\| = \|\epsilon_{t-1}\|_{\psi_2}^2 =   \mathcal{O}(\sigma^2)$ for $i=1,2,...,\theta$. The desirable result follows by setting $\mu = \mathcal{O}(\sqrt{\theta}\sigma)$.

% \subsection{Theorem 3}


% \begin{theorem*}
% \label{thm_Fourier_correct} 
% Let $A\in\mathbbm{R}^{d\times n}$ be the Fourier coefficients matrix of an input matrix $X\in\mathbbm{R}^{d\times n}$, and $\mu(A)$, the coherence measure of matrix $A$, is $\Omega(k/n)$. We assume there exist $s$ and  a positive $ a_{\min}$ such that the elements in last $n-s$ columns of $A$ is smaller than $a_{\min}$. If we keep first $s$ columns selected and randomly choose $\mathcal{O}(k^2/\epsilon^2 - s)$ columns from the remaining parts, with high probability
% \[
%     \|A - P(A)\|_F \leq \mathcal{O}\left[(1 + \epsilon)a_{\min}\cdot\sqrt{(n-s)d}\right],
% \]
% where  $P(A)$ denotes the matrix projecting $A$ onto the column selected column space.
% \end{theorem*}
% (In Theorem \ref{thm_Fourier_correct}, we correct a typo error in Theorem \ref{thm_Fourier}. The ``in last d - s columns...'' should be ``in last n - s columns...''). 

% \begin{proof}
% Similar to the analysis in Appendix C of~\cite{FedFormer}, let $A_k = P(A)$ and $A_{\bar{k}}$ be the matrix projecting A onto the remaining-column space, where the columns are not selected. $A = A_k + A_{\bar{k}}$. So we have $\|A - P(A)\|_F = \| A_{\bar{k}}\|$. In the assumption of Theorem \ref{thm_Fourier_correct}, the elements in $A_{\bar{k}}$ is smaller than $a_{\min}$, thus $\| A_{\bar{k}}\|_F = \sqrt{\mathrm{trace}(A_{\bar{k}}^\top \cdot A_{\bar{k}})} \leq a_{\min} \cdot \sqrt{(n-s)d}$. ($A_{\bar{k}} \in \mathbb{R}^{d \times (n-s)}$)
% \end{proof}
